# Supplementary material for: Costs and benefits of authentication advice
Source: arXiv:2008.05836 source file (2023-02-16)
Supplement: Supplementary file 1 [file appendix1.tex]

\section{Advice discussion}\label{sec:disc_adv}
%%%%%%%%%%%% Access

%%%%%%%%%%%%%%%% Administrator Accounts
\subsection{Administrator Accounts}
Administrator accounts are often managed using two protocols: su and sudo.  The su commands opens a new terminal into which the user can enter the password for the account they wish to access. To access an administrator account the administrator password must be provided. The sudo command allows a user to run a command with root permissions. The user types the password for their own account and if this account is in group wheel then it has permission to run a command as root. The four pieces of advice in this category unanimously recommend creating a clear distinction between administrator accounts with privileged access and normal user accounts.

%%%%%%%%%%%%%% Backup password options
\subsection{Backup password options}
The advice relating to backups for forgotten passwords refers to email, security questions and hints. All the advice is unanimous. 
Three organizations recommending the use of security questions. Schechter et al. show that security questions can be very easily guessed and are also easily forgotten by users \cite{schechter2009s}. ``Do not store hints'' is certainly considered to be good advice in light of the Adobe leak \cite{adobecrossword}. Both ``do not store hints'' and the requirement for security questions to be difficult to guess increases the forgettability for users. 

%%%%%%%%%%%%% Backup work
\subsection{Backup work}
One organization recommended making digital and physical back ups. This can save an organization a large amount of hardship if a breach or ransom attack occurs. 
% It takes time, computing memory, and resources in advance as the organization needs to save regular digital and physical back ups.

%%%%%%%%%%% Composition
\subsection{Composition}
Composition restrictions are regularly enforced by websites but the advice given is not consistent from site to site. Herley \cite{herley2009so} hypothesizes that different websites may deliberately have policies which are restrictive to different degrees as this can help ensure that users do not share passwords between sites. We have also heard this expressed by system administrators. Below we will discuss each of the three statements associated with composition. 

\paragraph{Must include special characters}
Seven sites instructed users to ``include special characters'' in their passwords, but five sites placed restrictions on which special characters can be used. A frequent restriction on special characters was ``do not use spaces". However, one piece of advice stated the more direct ``do not use special characters".

\paragraph{Don't repeat characters}
Not allowing the repetition of characters deters users from choosing passwords such as ``aaaaaaa" or ``wwddcc". Depending on the strictness of the restriction it could eliminate words such as ``bookkeeper" or ``goddessship".

\paragraph{Enforce restrictions on characters}
We collected twelve pieces of advice encouraging composition restrictions on passwords and only one piece of advice against it. The source rejecting composition rules was the NIST 2017 password guidelines. The guidelines are receiving a positive response from the research community \cite{nistcox}. This raises the question: will organizations begin to disseminate these new security practices? Or continue to enforce their stringent password restrictions?

We claim that forcing users to include special characters reduces the attackers total search space. If a user creates an eight digit passwords with no restrictions each of the eight characters could be any of the 96 possible ASCII characters. However, by restricting the password so that it must include one special character we limit the options for one of the character to the 34 special characters. This becomes more significant when a site enforces multiple restrictions on composition. In addition, the probability of a user including a ``1" as their number and an ``!" as there symbol is high \cite{ur2015added}. So again an attacker can refine the guesses they make. Abrams and Bulter find that Password policies that require a minimum character length and mandate the use of lowercase letters, uppercase letters, numbers and symbols may reduce the number of viable passwords by more than 60\% \cite{youtube_pwd_constraints}.

%%%%%%% Default Passwords
\subsection{Default Passwords}
Four organizations recommended changing all default passwords. Default passwords are used in Internet of Things devices and WiFi equipment among other things. Manufacturers  set  a default  password,  which  an administrator is supposed to change during setup \cite{farik2015analysis}. These default passwords are, in their essence, not secure as they are public knowledge. They have been shared publicly and often the same logins are using for many or all of the devices of that type manufactured by a given company. Changing the default password takes time during the set up of the device but once done should not need to be updated unless it is compromised.

%%%%%%%%%%%%% Expiry
\subsection{Expiry}
\paragraph{Unanimous}
We found five pieces of advice telling organizations to ``Store password history to eliminate reuse'', one encouraging organizations to ``Enforce a minimum password age'' and ten in favor of ``Changing passwords if compromise is suspected.''

The reason given for introducing a ``minimum password age'' is to prevent users from bypassing the password expiry system by entering a new password and then changing it right back to the old one \cite{technetmag}. 

Ten pieces of advice recommended ``changing passwords if a compromise is suspected''. This can be inconvenient for users not affected by the compromise, and also those who are. If there is a breach at the server the users were not at fault yet still they must choose a new password. 

\paragraph{Contradicting} 
From anecdotal evidence we know the advice ``change your password regularly'' is widely disliked by users \cite{hatechangingpass}. 
%XXX Referring to the costs in Table \ref{tab:costs}
When looking at our costs model it is worth noting that most costs are one-time occurrences but expiry costs are triggered periodically. Seven pieces of the advice we collected encouraged the use of password expiry while only four pieces of advice discouraged it. This is despite research suggesting that the security benefits are minimal \cite{chiasson2015quantifying}\cite{zhang2010security}. This implies the inconvenience to users is worth less to organizations than the minimal security benefits. Or do organizations want to be seen to be enforcing strong security practices, and forcing expiry is just one way of doing this?

%%%%%%%%%% Generated Passwords
\subsection{Generated Passwords}
\paragraph{Unanimous}
One piece of advice said that generated passwords must not be stored and one piece of advice said that generated passwords should only be valid for the users' first login. 

\paragraph{Contradicting} 
We have two contradictory advice statements in this category. One advises creating random passwords using a random bit generator. The contradicting advice says to generate passwords that aid memory retention. Random passwords are very difficult for users to remember \cite{zviran1993comparison} but passwords that aid memory retention can potentially lead to easier guessability.

%%%%%%%%%%%% Individual Accounts
\subsection{Individual Accounts}
Having one account per user with a password is important for maintaining access controls and also tracking errors or attacks back to a source account. The cost can be high in an environment where there are shared computers. In these scenarios, if work is switching between users each user must log in and out multiple times. In addition a company may need to pay per account they use and necessitating one account per user can significantly increase company costs.

%%%%%%%%%%%%%% Input
\subsection{Input}
\paragraph{Truncation}
One organization advised that truncation of the password should never be enforced. That is, if a user creates a 12 character password, the verifier should not decide to just  store and compare the first 6 characters for authentication. 

\paragraph{Accept all characters}
Only one organization argued for acceptance of all ASCII and UNICODE characters. But this same organization said that removing multiple consecutive space characters was acceptable. In the category \textit{Composition} we also saw this aversion to the space character. Consecutive spaces may be considered an error and a password made entirely of spaces could be considered weak, but no more so than repeating any other character is considered weak. If hashed, the space character would also result in a different hash value and therefore would add length and variety to a password. Allowing spaces could also encourage users to use passwords consisting of multiple words. 

%Keep accounts safe % ---do not include
\subsection{Keep accounts safe}
All the advice in this category was unanimous. It recommends a number of background defense strategies. 
``Implement defense in depth'' and ``apply technical defences'' are both vague pieces of advice but good in theory. They require a system layered with security. Technical defenses could potentially reduce the human cost factor. ``Monitor and analyze intrusions'' is a continuous job and often intrusion points are only discovered retrospectively.

%Keep your account safe
\subsection{Keep your account safe}
\paragraph{Check webpages for SSL}
This advice tells the user to check that the connection from the web server to the browser is encrypted usually by identifying the closed padlock in the URL bar. However Schechter et al found that 53\% of their study participants attempted to log in to a site after they were interrupted by a strong security warning. Likely even if users see a closed padlock, they would still continue to use the webpage \cite{schechter2007emperor}.

\paragraph{Manually type URLs}
Manually typing URLs can be very time consuming for users and the assortment of symbols included can make transcription difficult. Manually typing URLs means a user should not be fooled my a fake link. For example, a link \url{www.safe.com} which actually directs to \url{www.you-are-in-trouble.com}. Manually typing the URLs can lead to a typographical error and a malicious website could take advantage of this. For example a website called \url{www.faceboook.com} which masquerades as facebook and asks for login credentials. Only one piece of advice asked for URLs to be manually typed.

\paragraph{Don't open emails from strangers}
In certain jobs it can be impossible to not open email from strangers and even in everyday life it can be very inconvenient. 
However, a 2012 study by B{\"o}hme and Moore found that as a result of concerns over cybercrime 42\% of participants say they do not open email from strangers \cite{bohme2012consumers}. We only collected one piece of advice which said ``Don't open emails from strangers''.

\paragraph{Keep software updated \& keep antivirus updated}
Two places recommended these pieces of advice. In their paper ``Tales of Software Updates: The process of updating software'' Vaniea and Rashidi found that 49.3\% of respondents relayed negative experiences with software updates. This is likely similar for antivirus updates with the added disadvantage that antivirus may also need to be repurchased regularly.

\paragraph{Log out of public computers}
Finding the person before you on the public computer has not logged off can lead to different reactions. Some might take advantage and snoop around, maybe leave a message for the user to see to show they were vulnerable, or just log them off. But with this privileged access an opportunistic attack can do a lot of damage. Spending money with linked credit cards, masquerading as the user and asking for money to be transferred by the user's peers, and setting up backdoors into the accounts for future use, among other things. Despite the fact that we know these are threats we could find little evidence of reported breaches as a result of this. It is unclear whether this is because it does not occur or whether victims don't reveal or don't know that this as the reason for their breach.

\paragraph{Password protect your phone}
Nowadays users can conduct most online transactions via mobile phones. Their portability makes them susceptible to theft. Therefore password protecting a phone could be more important even that password protecting our computers. Yet because phones are carried on our person, it is likely that users are more likely to leave themselves continuously logged on to applications.

%%%%%%%%%% Length                                                                                                                                                                                                                                                                    
\subsection{Length}
\paragraph{Enforce a minimum password length}
Enforcing a minimum length inconveniences memorability and may force users to alter or change their password. If our aim is to minimize password reuse, then this might not necessarily be a draw back \cite{herley2009so}. A minimum length could also be seen as reducing the total search space of an attacker. However, it definitely has the advantage of restricting the use of zero or one character passwords. Most of the advice encouraged the minimum length to be set at eight characters, likely as a protection against GPU-based guessing.

\paragraph{Enforce maximum password length}
Three pieces of advice recommended enforcing a maximum password length: 15 characters \cite{intel}, 20 characters \cite{paypal} and 40 characters \cite{interactivebrokers}. Interestingly Paypal do not list maximum password strength as one of their restrictions. Only when a user attempts to enter their password is the restriction revealed. NIST 2017 guidelines \cite{nist2017} state that  ``Verifiers should permit subscriber-chosen memorized secrets at least 64 characters in length". Restricting the length of a password inconveniences personal systems for password generation, in particular it effects users who usually choose long passwords. It also restricts the outputs of a random password generators and introduces an upper bound on the attacker's search space.  
 
%On an interesting side note, from experience we know that many sites do not initially reveal what restrictions they are enforcing \cite{paypal}. Yet we found no advice recommending this practice.

%%%%%%%%%%%%%%%%%%%%%%%%%%% Multi factor authentication
\subsection{Multi-factor authentication}
\paragraph{Use multi-factor authentication}
Multi-factor authentication traditionally involves: \textit{something you are}, \textit{something you know}, and \textit{something you have}. Examples for each of these respectively are: fingerprint, password and a USB key token. One piece of advice recommended using multi-factor authentication. Using \textit{something you have} as one of the requirements for authentication means that the user may need to carry an additional item around with them. In addition, this item (unlike \textit{something you know} or \textit{something you are}) is easily susceptible to theft. If theft does occur though, the user is still nearly as secure as if the second factor had never been used. 

\paragraph{Use 2 step verification on phone}
Using a phone would count as the \textit{something you have} form of authentication. One piece of advice recommended this. Two step verification is different to multi-factor authentication in that the two steps could use the same factor. For example a fingerprint and facial recognition would be a valid authentication combination for two step verification but would not suffice for two factor authentication. 
Phones can be stolen or the code sent to the phone can be revealed by eavesdropping or a side channel attack. However if this occurs, depending on what is chosen as the second step, the users' account could still be secure. 

\paragraph{Use for remote accounts}
One piece of advice said to use multi-factor authentication for remote accounts. 
Remote accounts are often more vulnerable as the user might need to connect over an insecure channel. Therefore the multi-factor authentication process is seen as adding extra security to the account. It is more likely that the second factor will be compromised if used remotely; either by theft or by eavesdropping.

 %%%%%%%%%%%%%%%%%%%%%%%%%% Network: Community Strings
 \subsection{Network: Community Strings}
 A community string is a user ID or password that is sent along with an SNMP request \cite{hare2010simple}. A community string is a password for access to statistics within a device or router. Someone can access data from such devices if they know the correct community string. 
 
 \paragraph{Don't define as standard default}
 The standard default for community strings is set by the vendor. Vendors can choose the same password for all their devices and can have defaults passwords as simple as `public' \cite{jiang2002multiple}. These defaults are generally easily guessed. The community strings allow an attacker to find out about a organization's network and potentially find access points. This compares with the advice regarding the changing of all default passwords.

 \paragraph{Different to login password.}
Often community strings are not encrypted. Because they are transmitted in cleartext they can be read by anyone. This is an issue if the password sent is reused for other applications. This compares with the advice ``Don't transmit passwords in cleartext'' and ``Don't reuse a password''.

%%%%%%%%%%%%%%%%%%%%%%Password cracking
\subsection{Password cracking}
\paragraph{Attempt to crack passwords}
Administrators attempting to crack users passwords is a method for removing the ``low hanging fruit'' from attackers' reach. By requiring users to change their password if it was guessed by the administrator, the hope is that a stronger password will then be chosen by the user. This is a classic application of the original `crack' program \cite{muffett1992crack}. This is a common policy for organizations \cite{klein1990foiling}\cite{yan2001note}, yet only one piece of advice we collected recommended it. We speculate whether organizations are unwilling to openly admit and recommend this practice.

%%%%%%%%%%%%%%%%%%%%%%%%%%%%%%%%%Password managers
\subsection{Password managers}
\paragraph{Use a password manager}
Password managers are a convenient method for storing and auto-filling users' passwords. The single sign on means that users recall a single master password which is used to protect all other passwords. A password manager does mean that the user is relying on an external agent to store their passwords and therefore if this agent is compromised then the password of all accounts are compromised. \textcolor{red}{In their 2019 study, Zhang et al. found that users of password managers reported the initial set up taking a lot of work and that usability and compatibility issues exist, specifically when used on mobile devices \cite{zhang2019people}.}

\paragraph{Create long random passwords}
One piece of advice recommended that when a user is using a password manager they should ``create long random passwords''. Long random passwords are resilient to brute force guessing but generally are too much of a memory strain for users \cite{florencio2014password}. Where a password manager is saving the password for each use, the usability issues are no longer a concern.

%%%%%%%%%%%%%%%% Personal Information
\subsection{Personal information}
\paragraph{Unanimous}
Eight pieces of advice instruct against choosing passwords that match account information. If this restriction is enforced by an organization, an increase in computing power is needed as the password needs to be cross checked against the users' information. The advice is enforceable and protects against elementary targeted attacks. A simple form of this are `joe accounts', where the username and password match \cite{joeusers}. In 1989, Bishop and Klein cracked 40\% of 14,000 UNIX accounts using guesses derived from associated usernames or account numbers and dictionaries \cite{bishop1995improving}.

\paragraph{Contradicting}
The advice, ``don't include personal information in your password'' was issued by five sources. It is partially contradicted by the advice which says: ``Personal details such as spouse's name, vehicle license plate, PPS or social security number and birthday must not be used unless accompanied by additional unrelated characters" \cite{dcu}. It does not seem feasible to enforce this without cross referencing against some body of user information. However, if the advice is followed it would protect against a targeted attack. Castelluccia et al., find they can crack 5\%\ more passwords by leveraging personal information about users \cite{castelluccia2013privacy} and Li et al. discover that just over 60\% of passwords in their study of a Chinese password dataset contain at least one piece of personal information \cite{li2017personal}

Eight different sources advise against the inclusion of names in passwords, e.g. ``do not choose any common name" \cite{bostonuni}. However, one source contradicts this saying: Choose ``someone else's mother's maiden name (not your own mother's maiden name)" \cite{getsafeonline}. By not including your own mother maiden name a targeted attack will not be affected. However, it offers no protection from a bulk guessing attack. We consider a ban on names to be capable of eliminating a significant number of guesses for an attacker. In addition, words which double as names could be eliminated, ``Bob", ``Amber", ``Jack", as a result of this restriction.

%%%%%%%%%%%%%%% Personal password storage
\subsection{Personal password storage}
\paragraph{Unanimous}
Four sources advised users to ``not leave passwords in plain sight''. This advice is difficult or impossible for an organization to enforce. Shay et al., find that users are more likely to share and reuse their passwords than write them down \cite{shay2010encountering}.

Of the three sources warning against the use of the ``remember me'' option, two advised never using it, and one said never to use it on a public computer. By not using the ``remember me'' option, there is an increased need to remember passwords. Also, more user time is consumed, since the user now needs to enter their password every time. It does decrease the chance of an opportunistic or targeted attack. 

\paragraph{Contradicting}
Two sources told users to ``not store passwords in a plain text computer file'' and one source recommended that if you were doing it, a unique name should be chosen for the file so people don't know what's inside. This advice still shows an awareness of the risks of a targeted attack.

``Writing passwords down safely'' creates an additional security hole as the written password can now be compromised. In terms of usability, if a user forgets their password they need to take the time to retrieve their safe copy. However, the time cost for the user would be greater if the user has no backup copy of their password. Adams and Sasse \cite{adams1999users} conducted a survey of corporate password users and found them flustered by password requirements and coping by writing passwords down on post-it notes. Komanduri et al. \cite{komanduri2011passwords}  found that most participants in their study write down or otherwise store their passwords. Interestingly they also find that, storage is correlated with the use of higher-entropy passwords. In fact, some experts recommend writing passwords down as a mechanism to cope with numerous passwords \cite{schneierwritedown}. Shay et al. found that users are more likely to share and reuse their passwords than to write them down \cite{shay2010encountering}. We found six pieces of advice recommending that users write their passwords down safely, and one piece of advice discouraging it. 

%%%%%%%%%%%%% Phrases
\subsection{Phrases}
Advice regarding password phrases was the most commonly given advice we encountered. This implies that advice is mostly concerned with making passwords `strong'. While this is important for some attacks, for attacks such as phishing and keylogging the strength of the password is irrelevant \cite{zhang2016revisiting} \cite{florencio2016pushing}.

\paragraph{Unanimous}
Within the category \textit{Phrases} there were no contradictions for the statements: ``Don't use patterns, Take initials of a phrase'' and ``Don't use words.'' The last is particularly interesting since from leaked password database we know users primarily choose word based passwords \cite{rockyou}. Shay et al. find that the ``use of dictionary words and names are still the most common strategies for creating passwords" \cite{shay2010encountering}. This depicts how ineffective some password advice can be and is possibly a reflection on the costs appearing to not outweigh the benefits from a users' point of view. 

\paragraph{Contradicting}
The statements: ``Don't use published phrases'' and ``Substitute symbols for letters'' had contradictions. For ``don't use published phrases'' one piece of advice said ``Don't use song lyrics, quotes or anything else that has been published''. Another piece of advice said ``Choose a line of a song that other people would not associate with you''.
The second piece of advice directly contradicts the first. This inconsistency makes it no surprise that users seem disinclined to follow security advice \cite{inglesant2010true}\cite{adams1999users}.

The advice statement ``Substitute symbols for letters'' is proposed by two sources but is advised against by a third. We know from Warner \cite{subs} that passwords with simple character substitutions can be weak. Yet, 2 of 3 pieces of advice recommend it. This could stem from the attitude that it is `better than nothing'. 

%XXX and, as we can *will see later* see from Table \ref{tab:costs}, the cost to the user is relatively low. 

\subsection{Policies}
\paragraph{Establish clear policies}
Two places encouraged organizations to ``establish clear policies''. This is interesting since a lot of the advice we have collected is contradictory. Including the advice from those two organizations who gave this advice!

%%%%%%%%%%%%%%% Reuse
\subsection{Reuse}
We collected six pieces of advice telling users to ``never reuse passwords'' and three pieces telling users to ``not reuse passwords for certain sites''. In addition, we found three pieces of advice encouraging users to ``alter and reuse their passwords'' and three pieces telling users to not alter and reuse their passwords. There seems to be little agreement among the distributed advice in terms of password reuse. 

\paragraph{Never reuse a password vs. reuse for certain accounts}
Das et al. estimate that 43-51\% of users reuse passwords across sites \cite{das2014tangled}. They also provide algorithms that improve an attacker's ability to exploit this fact. Flor{\^e}ncio, Herley and Van Oorschot \cite{florencio2014password} declare that, ``far from being unallowable, password re-use is a necessary and sensible tool in managing a portfolio'' of credentials. They recommend grouping passwords according to their importance and reusing passwords only within those groups. Interestingly, the advice we collected ``Don't reuse certain passwords'' gave a slightly different take on this advice. The advice mostly asked users to not use the password used for their site anywhere else e.g. ``Never use your Apple ID password for other online accounts". Most organizations gave advice prioritizing their own accounts. Only one piece of advice suggested using a unique password for any important accounts \cite{google}.

\paragraph{Alter and reuse passwords}
An alternative to grouping accounts for reuse is to alter and then reuse a password. This advice was given by three sources and rejected by three sources. Alterations to password are often very predictable. Using a cross-site password guessing algorithm Das et al. \cite{das2014tangled} were able to guess approximately 10\% of non-identical password pairs in less than 10 attempts and approximately 30\% in less than 100 attempts. We could find no research suggesting this method of altering and reusing passwords as effective though anecdotally it is common \cite{stobert2014password}.

%%%%%%%%%%%%%%%%%%%%%%%%%%%%%%Sharing
\subsection{Sharing}
Nine pieces of advice said ``Never share your password''. Three specified not sharing by email and one specified not sharing over the phone. 

Weirich and Sasse find that sharing your password is regarded as a gesture of trust and refusing to share your password with someone is an indication that you do not trust them \cite{weirich2001persuasive}. A 2011 study of 122 people found that one third of respondents reported sharing their personal email password, a quarter shared their Facebook password and approximately 20\% of people who had work email passwords reported sharing them with colleagues \cite{kaye2011self}. However they do find that thought and consideration is given before the password is shared. This tells us that the user is aware of the security risks and may accept them on the ground of trust. 

%%%%%%%%%%%%%%%%%%%%%%%%%%%%%%Shoulder surfing
\subsection{Shoulder surfing}
\paragraph{Offer to display password}
One piece of advice recommended offering to display the users' password when they type it at login. Jacob Nielsen in 2009 challenged the masking of passwords \cite{nielsenmasking}. Bruce Schneier, after originally agreeing with the removal of masking, here \cite{schneiermasking} sums up why password masking needs to continue in certain contexts. 

\paragraph{Enter your password discretely}
This advice is unenforceable and relies on user education. Research has analyzed mitigations for the threat of a shoulder surfing attack \cite{kumar2007reducing}\cite{roth2004pin}. But Flor{\^e}ncio, Herley and Coskun suspect that shoulder surfing attacks are not very common as humans are very good at detecting people in their personal space \cite{florencio2007strong}. Eiband et al. find that shoulder surfing mainly occurs in an opportunistic, non-malicious way and it is usually personal data that is observed \cite{eiband2017understanding}.

%%%%%%%%%%%%%%%%%%%%%%%%%storage
\subsection{Storage}
\paragraph{Restrict access to password files. }
The advice in this category recommended encrypting the file the passwords are stored in and restricting access to those files. An example of this in practice is Unix's /etc/shadow file vervsus the /etc/password file. In the beginning the /etc/password file contained usernames, userids, description, passwords, and other information for users. The passwords were encrypted and the file was read only for anyone but the user. But encrypted passwords are susceptible to a dictionary attack, and the passwords could be read by all users so any of them could attempt this attack. 

The solution was to move the passwords out of /etc/password and into /etc/shadow. /etc/shadow is an encrypted folder which contains hashed and salted passwords. The owner has read and write permissions but not even read permission is granted to any other users on the system  (-rw- --- ---). This access controls are implemented in Unix and Linux machine and result in a secure out of the box authentication protocol. Yet restrictions on access to password files was encouraged by only 2 organizations and only one organization recommended encrypting password files. We discuss the methods used for storing passwords in more detail in the category ``Password Storage''

\paragraph{Encrypt passwords file}
This is the encryption, usually with a password as the key, of the file containing all the passwords. Encrypting this file means that when any user wishes to log in, the whole fill is decrypted, the password is compared to the value entered by the user, and then the file is encrypted again. Encrypting the individual password values is different and is discussed below.

\paragraph{Store password hashes}
Four pieces of advice recommended storing passwords as hashes. 
A cryptographic hash is a bit string of a fixed size which should uniquely represent a password. It is irreversible but is deterministic i.e. the same password will always map to the same hash. An attacker can discover the passwords by creating a large look up table (rainbow tables) which matches each password to a corresponding hash value. This is very effective for passwords up to a certain length and after this point a brute force search is still possible. Flor{\^e}ncio et al. provide a decision tree in their paper ``An Administrator’s Guide to Internet Password Research'' showing the attacks different methods of password storage are susceptible to \cite{florencio2014administrator}. 

Two of the pieces of advice recommending hashes also recommended using a salt. A salt is large random, non-secret nonce value which can be stored with the password hash. The salt randomizes the output of the password hash, making the use of rainbow tables impossible. An offline guessing attack is necessary for revealing the passwords. 

One piece of advice relating to salting said to use ``a unique salt for each account''. The second salt related piece of advice did not specify whether the same salt could be used for all accounts of whether a unique salt was to be used. If the same salt is used then a look up table is still a feasible attack.

\paragraph{Encrypt passwords}
Encryption of passwords was the first common method recommended as a means of protecting passwords \cite{morris1979password}. However it is often reversible and a key needs to be protected for security to be maintained. It is now recommended that the hashing and salting method is used for password storage. 

Despite this, seven pieces of advice recommended password encryption, in comparison to only four pieces of advice recommending hashing and only two recommending hashing and salting. Not specifying the use of a salt might be a careless use of terminology, but a 2019 paper by Ntantogian et al. found that 14.29\% of Content Management Services surveyed did not use a salt in their default hashing scheme \cite{ntantogian2019evaluation}.

In the case of a password leak, either the key is revealed along with the password database or it is not. If the key is revealed all passwords are immediately decryptable. If the key is not revealed then brute force guessing can be attempted against the key, but this is a difficult task. For example in the adobe breach, though most passwords were compromised by guessing, the key was never discovered \cite{adobe_guardian}.

\paragraph{Don't hardcoding passwords}
Hardcoding passwords will make is very difficult to automate changes making it a less usable method. Hardcoding will also make it less secure since it may be stored in plaintext to a file that an administrator can directly edit.

%%%%%%%%%%%%%%%%%%%%%%%%%Throttling
\subsection{Throttling}
\paragraph{Throttle password guesses}
To fight against online guessing, we can have a fixed or exponentially increasing delay after each failed authentication attempt. For example after 10 incorrect guesses the account is locked for 24 hours or until it is unlocked by an administrator. 

%%%%%%%%%%%%%%%%%%%%%%%%%%%%Transmitting passwords
\subsection{Transmitting passwords}
Four pieces of advice recommend not transmitting passwords in plaintext. This relates to the organization distributing passwords, either those that have been created by a user or those that they have generated for users. Two pieces of advice tell the organization to request passwords over a protected channel, for example when they are requesting a password at account creation. These are very similar pieces of advice since both groupings place the onus on the organization to oversee that passwords are sent by protected channels. 

If passwords are transmitted in clear text they are susceptible to any eavesdropper on the network. Let's Encrypt has in recent years helped to make security certificates accessible to more websites \cite{letsencrypt}. However providing a secure channel for passwords is not an easy task. In a 2017 2-hour lab study 18.5\% of educated participants failed to set up a secure HTTPS connection \cite{krombholz2017have}.

%%%%%%%%%%%%%%%%%%%%%%%%%%%%Username
\subsection{Username}
\paragraph{Enforce composition restrictions on usernames}
Flor{\^e}ncio, Herley and Coskun argue that it is better to increase the strength of the userID rather than the passwords \cite{florencio2007strong}. They propose that this will protect against online guessing attacks but will not majorly increase the cost to users since the username can be recorded visibly.

\paragraph{Don't reuse username}
If the same username is used for multiple accounts then once the password for one account is compromised, this password can be tried against the same person's other accounts. Das et al. find that 43-51\%,  of  users  directly  re-use  passwords between  sites and many others introduce small modifications to their passwords across sites \cite{das2014tangled}. Not reusing a username could be one way to protect against an attacker leveraging this vulnerability and could be less burdensome on the user than a restriction on altering and reusing passwords. However, many sites require an email address as a username and it is not reasonable to prohibit reuse of an email address. 

\subsection{Don't allow users to paste passwords}
There become a tradition of not allowing users to paste passwords. There is no clear evidence for the origin of this advice and users often questions why they are not allowed to paste their passwords into the password field  \cite{troypaste}. We wish to evaluate the costs and benefits of this advice in our model.
