# Supplementary material for: Costs and benefits of authentication advice
Source: arXiv:2008.05836 source file (2023-02-16)
Supplement: Supplementary file 2 [file appendix2.tex]

\section{Costs rationale}\label{sec: rationale_costs}
Below we will describe the assignment of costs to advice statements. This may be helpful for a reader as an insight into our assignment process or for clarity on particular cost assignments. Not all advice statements are discussed where this would be repetitive. Instead we discuss any statements which might require additional information for clarity and provide that here. 

\subsection{User advice statements}

\subsubsection{Backup password options}
\paragraph{Email up-to-date and secure}
Most organization can not practically check that each user has kept their email up-to-date and secure. For a compliant user, this is a continuous process and will cost the user their time.

\paragraph{Security answers difficult to guess}
It is unlikely an organization will be able to enforce this advice. One option could be to employ guessing and require users to change their answers if they have been guessed. But in reality a practice such as this would have its own additional costs associated with it. Security answers which are difficult to guess will likely be difficult to remember and will also take time for the user to create. 

\paragraph{Do not store hints}
This statement represents two pieces of advice. One of the pieces of advice tells organizations to not allow users to store a hint, and one tells a user to not store a hint. 
An organization is unlikely to be able to stop users from storing password hints. However they can opt to not provide the facility for it.
We look at the costs from the point of view of the advice aimed at the user, i.e. the user voluntarily following the advice to not store a  hint.

\subsubsection{Composition}
For all three advice statements in this category the same costs are identified. The organization uses small amounts of computing power to verify that the password meets the requirements. 

\paragraph{Don't repeat characters}
Not allowing the repetition of characters deters users from choosing passwords such as ``aaaaaaa'' or ``wwddcc''. Depending on the strictness of the restriction it could eliminate words such as ``bookkeeper'' or ``goddessship''. It could also cause some inconvenience for random password generators where the word ``Sdt2htTtd65c8h'' could be rejected.

\subsubsection{Keep your account safe}
All the advice in this category requires user time. ``Check web pages for SSL'', ``Manually type URLs'' and ``Don't open emails from strangers'' are marked as periodic as they need to be repeated regularly. 
Both ``Keep anti-virus updated'' and ``Keep software updated'' require \textit{additional computing power}. The \textit{additional resource} of anti-virus software is definitely needed for the former and it is possible additional resources are also needed for the latter. 
Both ``Log out of public computers'' and ``Password protect your phone'' have the potential to introduce an increased password memory burden on users. 

The organization does not have the ability to enforce most of this advice. We mark it as voluntary for the users to follow. Alternatively, we could introduce organization time costs for the time spent on user education.

\subsubsection{Multi-factor authentication}
\paragraph{Use multi-factor authentication}
It is likely that either the user or the organization will have to provide the \textit{additional resource needed }for authentication, for example a USB token. We underline this cost as it depends on the implementation whether it is the user or the organization who must purchase the additional resources. 

\textit{Additional user time} is needed to complete the authentication process since multiple factors are needed at each login. Some devices do offer a ``remember me on this device option'' which would ease the burden on the users. But this will have it's own security trade-offs.  

Multi-factor authentication will require \textit{additional computing power} for both the user and the organization to authenticate someone with multiple factors.
If the user is using `something you have' to authenticate and loses it, this will also have an impact for \textit{user time and inconvenience}. Also, the user must remember to bring the device with them.

\paragraph{Use for remote accounts}
The costs for this piece of advice are similar to those for ``Use multi-factor authentication''. The difference is that the costs only need to apply to remote accounts. It does require the same amount of organization time to implement.

\subsubsection{Password managers}
\paragraph{Use a password manager}
A password manager helps a user by remembering their passwords and saves the user the time of typing the password at each site. A password manager will use some computing power. Some organizations will be able to force all their users to use a password manger but most organizations will not have this capability. This requires additional resources for the user as the user may need to purchase and/or download and maintain a password manager.

\paragraph{Create long random passwords when using a password manager}
One of the advantages of a password manager is that, because a user no longer needs to recall their passwords, the password can be as long and complex as a user wishes. Creating long and random passwords takes computing time and the user may need to specially configure the password manager. An organization specifying the type of password that should be created will inconvenience the users' personal system for password generation. If the password created is different to the users' general structure and is random, the user may never be able to remember it. This is only an issue if the password manager fails, the master password is forgotten or the user needs to access the account from a device not linked to the password manager.

\subsubsection{Personal Information}
\paragraph{Don’t include personal information}
This is a difficult thing for an organization to enforce. In fact, there is no reasonable way for an organization to eliminate all personal information from passwords. Some basic form of cross checking between user information could be done. For example, at the client end it could be possible to sweep the information on a device to ensure it is not included. Doing this has high organization and user end computing costs as well as privacy/GDPR implications. It also has the potential to inconvenience the users' personal system for password generation. There is also an \textit{Increased risk of forgetting} as personal details could have made the password more memorable. 

\paragraph{Must not match account details} 
An increase in computing power is needed to enforce this as the password needs to be cross checked against the user's information.

\paragraph{Do not include names}
We consider a ban on names to be capable of eliminating a significant number of options for users' passwords. This can \textit{Inconveniences users' personal system for password generation} and make passwords more difficult to remember.

\subsubsection{Personal Password Storage}
\paragraph{Don't leave in plain sight}
If the users are internal to the organization and work areas are monitored then it could be possible for an organization to enforce this advice. However in many situations it will be impossible. If the user follows the advice they have two options. They can memorize the password in which case there is a chance it is forgotten. Or they can store it in a hidden location which will require extra user effort or time to retrieve. This cost will take effect at every login as the user will need to check the password each time. 

\paragraph{Write down safely}
Encouraging users to write their password down means they are less likely to forget it. Therefore this is a positive for the cost category \textit{Increased risk of forgetting}. It is not particularly enforceable by the organization and will require user time to record the password and check it at each login. 

\paragraph{Don't choose ``remember me''}
The user will now need to remember their password instead of it being saved in the browser. In addition at each login the user will need to physically type their password.

\subsubsection{Phrases}
Needing to Blacklist common words or remove all patterns during password creation could be computationally expensive for the organization if the list becomes very large.  There exists a PAM module called `cracklib' which automates blacklisting \cite{muffet1997cracklib}.

``Take initials of a phrase'' and ``Substitute symbols for letters'' are both impossible to enforce. Unless an organization automates password generation, it is difficult to enforce ``Insert random numbers and symbols''. If it was automated it would carry little to no security benefits since it would be a known procedure.

\subsubsection{Reuse}
\paragraph{Never reuse a password} 
If users never reuse a password they must create a new password when they open the account. Because we are looking at a snapshot for a particular organization we assume users will have just one account in the lifetime. Therefore we do not mark this as having repeating costs though from a users' perspective it does. 

Password reuse could be within an organization or across organizations. It is very hard to enforce a no reuse policy across organizations. 

\paragraph{Alter and reuse passwords}
Specifying the structure that passwords should take could partially affect users' personal system for password generation.

\subsubsection{Username}
\paragraph{Enforce restrictions on characters}
We mark this as requiring the cost \textit{Inconveniences users' personal system for password generation}. While it is not a password, the advice does inconvenience the users' personal system for generating a username and, as such, could have similar costs.

\subsection{Organization advice statements}
%%%%%%%%%%%%%%%%%%%%%%%%%%%%%%%%%%%%%%%%%%%%%%%%%%%%%%%%%%%%%%%%%%%%%%%%%%%

%\subsubsection{Access to password file}

\subsubsection{Administrator Accounts}

\paragraph{Not for everyday use}
 The main cost here is to the administrator who must switch between accounts for different tasks. Though this burden is lessened by the implementation of programs such as su and sudo which allow users to easily run programs which require extra security privileges. In the time constraint we consider the administrator to be a user. The organization must also have the resources to create two accounts for the one user. 

\paragraph{Must have its own password}
This requires the organization to set up password protection on the administrator account. The administrator must create a new password and enter it in some way at each login. Multiple users with privileged access may all need to know the same administrator password. This is the disadvantage of using su protocols over sudo. 

\paragraph{Should have extra protection}
This advice is so vague that it is impossible for us to determine what exact costs are associated with it. We can assume that the organization will need to set these extra protections in place. It is likely to take time for the user, but with out knowing what the protections are we cannot say. Both sudo and su provide additional protection for administrator accounts.

\subsubsection{Default passwords}
\paragraph{Change all default passwords}
This requires changing from default passwords but does not require that each password is unique and they often may be recorded, thus not requiring much additional burden on users. The most inconvenient aspect would be identifying all the default passwords that are in use the technology used by the organization. Often administrator accounts exist on devices and have associated default passwords that the user of the device may know nothing about.

\subsubsection{Expiry}
\paragraph{Store history to eliminate reuse }
The organization must store all previous passwords, requiring memory. The user will need to pick a new password as old passwords cannot be reused. At creation the server must query the stored dataset to verify the uniqueness of the new password. There is also an \textit{Increased risk of forgetting} as the user may forget which passwords have been expired and which is the current password in use.

\paragraph{Change your password regularly}
Organizations will need to notify users of the requirement to change their password. The organization will need to update their stored dataset of passwords at each update. 
Because passwords regularly need to be changed we anticipate an increase in the memory load over time. Users will repeatedly \textit{need to choose a new password}. On top of this will be an \textit{increased risk of forgetting} as a result of the repeated changes. 

\paragraph{Change if suspect compromise}
The advice under this statement was ambiguous as to whether it was being aimed at a user or at an organization. We have chosen to interpret it as if it is aimed towards an organization. In this way the statement tells an organization that if they become aware of a compromise they should ensure that their users' passwords are changed. This is the correct interpretation for five of the ten pieces of advice in the category. It is also a more interesting way to interpret advice as the advice aimed at the user is unenforceable. 

An organization can either internally monitor breaches or link with a breach application. For example receiving notifications about their users' credentials from \url{https://haveibeenpwned.com} \cite{haveibeenpwned}. The notifications to users then will require organization time and updating password files will require computing power.

\subsubsection{Generated passwords}
\paragraph{Must be issued immediately}
Uses users time as the user must be available to receive the newly created password. Takes administrator time to distribute.

\paragraph{Only valid for first login}
Requires the user to generate their own password as well as administrators to generate the initial generated password. 

\subsubsection{Individual accounts}
\paragraph{One account per user}
This will require organization time to set up and resources to provide server space for the account. Different users using the same device will need to switch between their accounts, this logging in and out will cost the organization computing power and the user time.

\subsubsection{Input}
\paragraph{Don't performed truncation}
There will be an increase in computing power for hashing the additional characters and the user must now enter their entire password correctly each time. As a comparison also see the costs and benefits assosiated with setting a maximum password length.

\paragraph{Accept all characters}
The organization must create a system which has the ability to accept all characters in a consistent way. This is a non trivial task. It will involve the standardization of Unicode characters entered from any keyboard at each login. Accepting all characters reduces the likelihood that the policy will inconvenience a user's password choice.

\subsubsection{Keep accounts safe}
\paragraph{Implement Defense in Depth}
Because we do not know what defense in depth strategies would be deployed, we cannot fully capture the costs. We can say that the defense in depth will require organizational time to put in place.

\subsubsection{Length}
\paragraph{Minimum password length}
This advice \textit{increases the risk of forgetting} simply because the user needs to remember more characters. It also \textit{inconveniences  the users' personal system for password generation} as a user may not be able to use a password within their normal structure. 

\paragraph{Enforce maximum length (\textless40) }
This advice \textit{inconveniences  the users' personal system for password generation} as a user may wish to choose a longer password. In fact one of the pieces of advice we collected, told the organization to limit the password length to less than 15 characters. This inconvenience will also increase the chance that the user forgets the password. There is no additional reason for this advice to hinder memory and therefore \textit{increased risk of forgetting} is not marked in it's own right. 

Enforcing a maximum length saves on encrypting and sending a very long password. This would be a reduction in computing time. But needing to check the length requires a very small increase in the computing time. We say that these cancel out and any overall impact this advice has on the computing power is small.

\subsubsection{Network: Community strings}
\paragraph{Different to login password}
The user needs to create a new password. The community strings are often stored in configuration files and do not need to be memorized by the user.

\subsubsection{Shoulder surfing}
\paragraph{Offer to display password}
A visual image of the passwords could help users with the memorization of their password or users with difficulty typing. Therefore this advice has a positive effect on memorability and user inconvenience.

\paragraph{Enter your password discretely}
When a user is logging in it may take some extra time or inconvenience for them to verify that they are entering their password discretely.

\subsubsection{Storage}
\paragraph{Encrypt password files}
Encryption and decryption  may slow down the authentication process for the user. For the organization, at each system start up the password needs to be provided. This can be done manually, which would require periodic organization time. Or it could be automated in which case the password is accessible to the computer system, which would bear security risks, by reducing the effective secrecy provided by the encryption.

\paragraph{Store password hashes}
If the hash of the password is stored, then if the user forgets their password, the password cannot be recovered from the hash. Therefore the user will need to create a new password.

\subsubsection{Throttling}

\paragraph{Throttle password guesses}
Throttling involves limiting the number of wrong guesses that can be made against an account. The cost of this is that a legitimate user could accidentally be locked out if they mistype or forget their password a certain number of times.  For example, Brostoff and Sasse \cite{brostoff2003ten} find that with a three  strike system  31\% of users are unfairly locked out is.  With ten strikes it is 7\%. Smart systems can help to minimize the risk for real users \cite{microsoft_sync}.

\subsubsection{Don't allow users to paste passwords}
This advice has 4 different costs: the organization must implement it, the user must take the extra time to manually type the password, many password managers cannot function without pasting, users are at a much higher risk of typos, and a user may need to choose a much shorter password if they cannot simply paste it efficiently into the web-form at login. Also, often the user has already created their password before this rule is revealed.

\section{Benefits rationale}\label{sec: rationale_benefits}

\subsection{User advice statements}

\subsubsection{Back up password options}
\paragraph{Email up-to-date and secure. }
Email is used for password reset links and often as the method that a generated password is passed to users. Therefore having a secure email account can help against eavesdropping of passwords by attackers. It can also prevent unauthorized binding of a new password to a users' account through the form of an emailed password reset. Having an up-to-date and secure email system with a working spam/malware filter can help to protect against phishing and pharming attacks and compromise of an endpoint due to malware.

\paragraph{Do not store hints}
If hints were stolen then these hints could be used to facilitate online or offline guessing or to aid a social engineering attack. 

\subsubsection{Composition}
\paragraph{Enforce restrictions on characters}
Researchers have shown that having complex password composition rules can make the resulting passwords more difficult to guess \cite{kelley2012guess}. Though simply allowing only long (greater than 16 characters) passwords has a similar effect on guessability and may not cause as much hardship for users  \cite{kelley2012guess}. Having very stringent composition rules does have the effect of limiting the search space an attacker needs to look through. For example, a brute force exhaustive attacker has to search more possibilities for a password with 8 characters made up only of lowercase letters, than for an 8 characters password which has to have two numbers, two uppercase letters, two lower case letters and two symbols. This gap increases further if the user voluntarily chooses from all 95 possible character options.

\subsubsection{Keep your account safe}
\paragraph{Check web pages for SSL}
This task helps users verify that communications to this webpage will be transmitted securely with encryption. This will help to combat phishing and pharming since phishing and pharming sites usually do not use SSL encryption. However, Dhamija et al. found that 23\%  of  their  participants  did  not  look  at  browser-based cues  such  as  the  address  bar,  status  bar  or  security indicators \cite{dhamija2006phishing}.

\paragraph{Manually type URLs}
Manually typing URLs can save a user from a Phishing attack as the user should recognize that the URL is not linking to the correct website. However, manually typing URLs makes a user vulnerable to typo-squatting/URL hijacking \cite{szurdi2014long} e.g., \url{www.goggle.com}. A user is sent to the site with the similar URL which masquerades as the website of the user's intended destination. The site can then ask the user to enter their login details and store them to use on the real site. Thus the user's password is duplicated. 

\paragraph{Keep software updated}
By keeping software updated a user gains protection against vulnerabilities as soon as the patch is released. This can save a user from eavesdropping, side channel and endpoint compromise. %online guessing? 

\paragraph{Log out of public computers}
If a user does not log out of a public computer then the only protection a user has is the moral compass of the next person person who uses that computer. In this way a user's account can already be thought of as in a state of compromise. It is not obvious which of the 11 categories this opportunist attack comes under. We will somewhat arbitrarily place it under Eavesdropping. 

\paragraph{Password protect your phone}
If a phone is password protected then the probability of endpoint compromise is lower.

\subsubsection{Multi-factor authentication}
\paragraph{Use Multi-factor authentication}
As mentioned before multi-factor authentication traditionally involves: \textit{something you are}, \textit{something you know}, and \textit{something you have}. The \textit{something you have} is susceptible to theft. However, if it is stolen the user if still protected by their other authentication factor. Using multi-factor authentication decreases the success of phishing (as second factors are often not subject to replay) and online guessing attacks (as both factors must be guessed). We underline some of the benefits as it depends on which factors the user or organization choose to use. 

\paragraph{Use 2-step verification on phone}
The phone can be stolen or the code can be revealed by eavesdropping or a side channel attack. But again, if the phone is compromised, it is possible that the first step of the authentication process will keep the users' account secure. 2-step verification decreases the success of an online guessing attack and a phishing attack.  

\paragraph{Use for remote accounts}
Without knowledge of a specific second factor it is hard to say what the security effects are. Therefore, depending on what the second factor is, there is the potential for physical theft or endpoint compromise to jeopardize the authentication. The probability of the exchange being eavesdropped is much higher if used for remote accounts.

\subsubsection{Password managers}
\paragraph{Use a password manager}
If we assume the norm is for users to memorize their passwords, then a password manager does not, in its own right, offer additional security. It does greatly reduce the users' memory load and by extension then a user can use as long, random and complex of a password as they wish. Thus this act will increase security but just using the password manager does not guarantee users will increase the complexity of their passwords. A password manager does mean that the user is relying on an external agent to store their passwords and therefore if this agent is compromised then the passwords of all accounts are compromised. Therefore we consider this to be a new way in which the users' password can be duplicated. 

Password managers which automatically fill in the users' credentials with no user interaction do have some corner case vulnerabilities \cite{silver2014password}. Though this same paper shows that a password manager can provide more security that the normal manual typing of the password. But it does depend on the set up of the specific password manager. 

\paragraph{Create long random passwords}
This piece of advice was given in the context of a password manager. ``Configure your password manager to create 30--50 random characters with a mixture of upper- and lower-case letters, numbers, and symbols.'' It has the same benefits as creating a complex long password but without the user memory costs.

\subsubsection{Personal password storage}
\paragraph{Don't store in a computer file.}
An attacker accessing this password file can duplicate the password. %If the laptop or computer is stolen the password file would also be taken.

\paragraph{Write down safely}
Even if the password is stored safely, the very act of writing it down makes it's duplication and physical theft possible. There is discussion as to whether the security risks of writing passwords are in fact very low \cite{schneierwritedown}. And in fact, if users write down passwords, then they may be more confident making stronger password choices \cite{cheswick2013rethinking}\cite{komanduri2011passwords}\cite{herley2009so}.

\paragraph{Don't choose ``remember me''.}
If the ``remember me'' option is not used then if an attacker steals a laptop or computer they should not automatically have access to the accounts on it. It is equivalent to not logging out of an account.

\subsubsection{Reuse}
\paragraph{Never reuse a password}
Reusing passwords has the security disadvantage that if an attacker compromises a password on one site then the password can be used to gain access to other sites. 
This means if passwords are reused then online and offline guessing becomes much easier for an attacker. In fact, if the password is leaked elsewhere the chance of it being compromised for this given organization is just equal to be chance that an attacker tries. 
%phishing and pharming and social engineering attacks?

However, even with different passwords at different sites, the attacker has a good chance of being able to leverage the information from a separate compromised site to mount effective phishing, social engineering and guessing attacks \cite{das2014tangled}. These will be at a higher cost to the attacker though.

\paragraph{Alter and reuse passwords }
Altering and reusing passwords means not directly reusing passwords between sites. It will make a guessing attack necessary for an attacker even if they have access to a password belonging to the same user from a different site. However, Das et al. \cite{das2014tangled} were able to guess approximately 10\% of non-identical password pairs in less than 10 attempts and approximately 30\% in less than 100 attempts. Therefore we mark it as a limited security improvement. 

\paragraph{Don't reuse certain passwords.}
Asking users to not reuse certain passwords is equivalent to saying that a user can reuse some passwords. 

In fact, if we look at the specific advice in this category we can see that most organizations are asking users to not reuse the password for \emph{their} site. This does provide some security advantage as the attacker will not be able to directly access the protected account using the revealed password. But, as with ``don't reuse you passwords'' we know that an attacker can still leverage information from other compromised sites to attempt phishing, social engineering and guessing attacks.

\subsubsection{Sharing}
\paragraph{Never share your password}
In the process of sharing a password it could be eavesdropped. Not allowing users to share their passwords also helps to protect against social engineering. Though this is through the form of user education. 

\subsection{Organization advice statements}

\subsubsection{Access to password file}
\paragraph{Encrypt password files}
Encrypting password files will protect against the theft of the hard drive. However, the password used for encryption could still be read from the RAM. If the system can access the password without manual intervention then the password is likely to be stolen if the encrypted file is stolen. An attacker will have more difficulty downloading the password file for offline guessing. 

\paragraph{Restrict access to password files}
Restricting access to password files will protect against certain types of unauthorized binding. If an attacker does not have access to the stored authentication details then the attacker will find it difficult to change the password stored for the user or link additional passwords or authenticators to the account. Preventing read access to a password file could prevent offline guessing attacks. 

\subsubsection{Administrator accounts}
\paragraph{Not for everyday use}
It can be argued that the more times the authentication process is completed by the user, the more times it is susceptible to compromise during entry or transmission. 
We therefore say that not logging into the administrator account for everyday tasks decreases the chance of eavesdropping and side channel attacks.

\paragraph{Must have its own password}
If there is one administrator then ensuring that this administrator account has a distinct password means it is less vulnerable to eavesdropping and side channel attacks. However in most situations, many users will require privileged administrator access. In this case the problem depends on how you choose to implement this advice. If users access the administrator privileges by typing the administrator password via su then all privileged users must know the same password. This makes social engineering, phishing and endpoint compromise more likely.  In addition if multiple users are recording or sharing with others the same credentials then they are more likely to be duplicated and fall into the hands of an attacker. 

Alternatively, there might be administrative access via the user's own password (e.g. via sudo) or a second administrative account/password corresponding to each user with administrative privileges. 

All of these have associated security risks. In our table we have represented the case where there is one administrator who must create a second password which allows them access to administrator privileges. 

\paragraph{Should have extra protection}
Depending on the extra protection the account is given this will have different benefits.

\subsubsection{Backup work}
\paragraph{Make digital \&\ physical back-ups}
Having a back up of work means that attacks can be less harmful to the organization. Having backups does not directly decrease the chance of an attack but would be factored in in relation to the costs of a breach. Having physical backups of work does mean that the potential for physical theft now exists.

\subsubsection{Expiry}
\paragraph{Store History to eliminate reuse}
This advice is given alongside ``Change your password regularly''. The password must now also not match any previous passwords. This means that knowledge of old passwords will not directly lead to an attacker knowing a current password.

However, even though users can no longer reuse prior passwords, alterations are still possible \cite{shay2010encountering}. In fact, Zhang, Monrose and Reiter \cite{zhang2010security} identify that we can easily predict new passwords from old when password aging policies force updates.

In addition, if an attacker gains access to a users' account and changes their password, the user will be unable to change it again until the required number of days have elapsed, or with an administrator's help.

Finally, storing the history means there is an additional password file which needs to be protected. Because of the close relationship between old and new passwords \cite{zhang2010security}, if this file is revealed then the information
in it can be used to effectively guess the current password \cite{das2014tangled}.  

\paragraph{Change your password regularly}
In a certain situation changing your password regularly does decrease the probability of success of online guessing. Imagine an attacker cycling through a list of guesses. If a password is changed to something new during this guessing, then an attacker wishing to guess it must start their guessing process again from scratch. 

However, most attackers will guess the most probable guesses first and since passwords follow a long tailed distribution \cite{murray2018exploring,malone2012investigating} a rational attacker will typically stop and move onto a new account if the password is not captured within the first few million guesses. 

If the attacker correctly guesses the password within the time frame. Then the password will be changed at the beginning of the new period. This does bring some additional security but in reality once an attacker has access to the account they can set up a backdoor and will not need the password in future. Even if the attacker creates no backdoor the probability that they can guess the next period's password is high as users base their next password heavily on their previous password \cite{zhang2010security,das2014tangled}. Therefore, knowledge of the password from one period will strongly aid the attacker in guessing subsequent passwords.

\paragraph{Change if suspect compromise}
If the password has been leaked elsewhere then the advice is to change your password. This protects you from online or offline guessing attacks as otherwise an attacker with access to compromised password has immediate access to the account. Some of the caveats discussed above still apply. But the hope is that if a compromise is suspected, a user may be less likely to create a new password very similar to their old one. In addition the time scale to the creation of backdoor may be longer.

\subsubsection{Generated passwords}
\paragraph{Must be issued immediately}
This decreases the chance that generated passwords are stolen before they are told to the user. If passwords were created in advance they would likely be recorded as administrators could not remember multiple generated passwords. Therefore these passwords could be duplicated while in storage.

\paragraph{Distribute in a sealed envelope} 
This increases the chance that the password is physically stolen as the envelope could be taken. The password could also be duplicated since it has been recorded. If an adversary opens the envelope and duplicates the password then it will go undiscovered if the adversary places the password page in a new envelope and reseals it. The benefit of the sealed envelope is that an observational, audible or network eavesdropping attack is less likely. 

\paragraph{Only valid for first login} 
Because these generated passwords are often issued and created by administrators the user has no confidence in the security of their password up until the point they receive it. Maintaining a rule that passwords must be changed at first login means that the user can now have complete control over the security of this new password. This advice then protects against previous duplication of the password.

\subsubsection{Individual accounts}
\paragraph{One account per user}
The alternative is multiple users using the one account. With multiple users using the same account one user could modify the authentication information without informing other users (unauthorized binding). In addition, if multiple users are recording or sharing with others the same credentials, then they are more likely to be duplicated and fall into the hands of an attacker. Social engineering and phishing attacks and endpoint compromise are also more likely if there are multiple points of access.

\paragraph{Each account password protected}
If there is no password we can likely consider the account to already be in a state of compromise. Password protecting an account increases the security of the account by necessitating one of the attacks to take place before an attacker can gain access. It obviously protects against both online and offline guessing. In addition having a password makes a side channel attack more complex. An attacker should be able to differentiate the difference between an account login where no password is used and when a password is used.
%not end pt com
%not physical theft
%offline guessing -yes DING{58}
%side channel - sending no password looks different from sending a password. potentially \down
%online guessing - yesDING{58}
%

\subsubsection{Input}
\paragraph{Don't performed truncation}
Truncating passwords makes online and offline guessing easier. It can also affect social engineering attacks. If the user does not know that the password will be truncated they may reveal the first few characters of the password without realizing the true security extent of this action. 

\paragraph{Accept all characters}
This increases the necessary search space of an attacker attempting online or offline guessing. Allowing all characters could give more scope for a SQL injection attack, but the hope is that there would be adequate string escaping in place to mitigate this fear. We account for the implementation difficulties in costs.

\subsubsection{Keep accounts safe}
\paragraph{Implement Defense in Depth}
Defense in depth can be divided into three categories: physical controls, technical controls and administrative controls. The security defense in depth can provide depends on exactly what strategies are deployed. They have the potential to mitigate any of the eleven attack types but without knowing what is implemented we cannot say exactly what the security advantages or disadvantages are.

\paragraph{Implement Technical Defenses}
The same argument as above can be used for this advice; it is not specific enough for us to know it's benefits. Though it is unlikely to aid against physical theft and social engineering. 

\paragraph{Apply access control systems}
Access controls make sure that only certain users have access to their required aspects of the system. With respect to authentication, this means that only the privileged administrators have the power to view and control the authentication procedures and modify the stored authentication data. This protects against a malicious employee ``turning off'' authentication or other security mechanics, duplicating the stored password dataset or downloading malware to attempt side channel or keylogging attacks. However, exactly what this advice protects against depends on which specific access controls are put in place. 

\paragraph{Monitor and analyze intrusions}
Awareness of what an attacker is doing within the system and learning where the vulnerability is is important for security. However this advice has no direct security affect unless the analysis is acted on. For example, if an administrator witnesses an attacker duplicating the plaintext password file, then a forced password change might need to be implemented. Else if an administrator witness an attacker binding an additional form of authentication to a user or changing the credentials for a user, then these actions would need to be reversed. Monitoring and analyzing intrusions could also guide user education. 

%\paragraph{Regularly apply security patches}%aaa

\subsubsection{Length}
\paragraph{Minimum password length}
Inhibits brute force guessing as there are no passwords to guess with a very small number of characters, which are sometimes favoured by both users and guessers. 

\paragraph{Enforce maximum length (\textless40)}
Requiring that passwords are less than a certain number of characters makes them easier for an eavesdropper to record them as they are less likely to cross packet boundaries. It also makes online and offline guessing easier as the attacker now need only guess passwords within the given range. 

\subsubsection{Policies}
\paragraph{Establish clear policies}
This advice does not directly increasing or decrease the probability of success of an attack type.  

\subsubsection{Throttling}
Throttling (or rate limiting) password guesses drastically reduces the number of guesses an attacker can make. The attacker can no longer continuously make guesses until the correct password is accepted. However, because of the right-skewed nature of password distribution, the attacker does still have a high probability of success with a small number of guesses \cite{malone2012investigating}\cite{murray2018exploring}.

\subsubsection{Don't allow users to paste passwords}
There appears to be no security benefits to this advice \cite{sachapaste} and indeed in our model we cannot find any attack type that it mitigates.
