# Supplementary material for: Costs and benefits of authentication advice
Source: arXiv:2008.05836 source file (2023-02-16)
Supplement: Supplementary file 3 [file appendix_combined.tex]

\section{Advice: Costs, benefits and characteristics}\label{app:comb}
\subsection{Administrator accounts}
The advice in this category relates to access controls. The four pieces of advice in this category recommend creating a clear distinction between administrator accounts with privileged access and normal user accounts. This means an administrator must switch between their privileged and general user account depending on their current task. This could be time consuming for an administrator though the burden is lessened by the implementation of programs such as su and sudo which allow users to easily run programs which require extra security privileges. It can be argued that the more times the authentication process is completed by the user, the more times it is susceptible to compromise during entry or transmission. Therefore not logging into the administrator account for everyday tasks decreases the chance of eavesdropping and side channel attacks. Administrators agreed with all the advice statements in this category. One administrator respondent said ``Admin accounts should be used for the minimum amount of time necessary and then logged out. Very easy to compromise a system while logged in as an admin and then being tricked into executing malware''.

\subsection{Backup password options}
\paragraph{Email up-to-date and secure}
Email is used for password reset links and often as the method that a generated password is passed to users. Therefore having a secure email account can help against eavesdropping and can prevent unauthorized binding of a new password to a users' account through the form of an emailed password reset. Having an up-to-date and secure email system with a working spam/malware filter can help to protect against phishing and pharming attacks and compromise of an endpoint due to malware. In our user study, users were divided about whether this has no cost or a minor periodic cost. We suspect that for most users their email client will automatically update the email software. However, we do mark it as a minor periodic cost. Administrators also marked this as advice as having no cost. This reinforces the automated nature of email updates which will often be handler by the external email client.

\paragraph{Security answers difficult to guess}
Three organizations recommending the use of security questions. Schechter et al. show that security questions can be very easily guessed and are also easily forgotten by users \cite{schechter2009s}. 
Making security answers difficult to guess is a challenging task for an organisation. Administrators noted a large number of costs associated with the advice. Most notable is major user education periodically. Respondent to our user survey indicated that security answers which are difficult to guess will likely be difficult to remember and will also take time for the user to create.

\paragraph{Do not store hints}
If hints were stolen then these hints could be used to facilitate online or offline guessing or to aid a social engineering attack; for example, in the Adobe compromise \cite{adobecrossword}.
An organization is unlikely to be able to stop users from storing password hints. However, they can opt to not provide the facility for it. Administrators in our survey were asked ``Users should not set password hints on websites'' and end-users were asked ``Do not store hints about your password''. The major cost for users was that their password would be less easy to remember and that it would require extra time or effort. For the organisation the major cost is periodic user education. 

%%%%%%%%%%%%%%%%%%%%%%%%%%%%%%%%%%%%%%%%%%%%%%%%%%%%%%%
\subsection{Backup work}
We asked both users and administrators about the costs of needing to digitally and physically backing up work. From a user point of view it was their own work. From an organisation point of view it is the organisation's files and data. For both it requires time and resources. For the organisation there is also a need for user education and help desk support if a back-up policy is in place. Digital and physical back ups can save an organization a large amount of hardship if a breach or ransom attack occurs. However, backups do not directly decrease the chance of an attack. In fact, having physical backups of work does mean that the potential for physical theft now exists.

%%%%%%%%%%%%%%%%%%%%%%%%%%%%%%%%%%%%%%%%%%%%%%%%%%%%%%%
\subsection{Composition}
Though there are three pieces of advice in this category, we only asked users and administrators about the specific advice: ``Include specific character types in your password. E.g. your password must include uppercase, lowercase, digit, symbol''. This allowed us to reduced the number of questions in our survey. We believe the costs for the other statements can be extrapolated from the responses we did receive. 

\paragraph{Must include special characters}
Seven sites instructed users to ``include special characters'' in their passwords, but five sites placed restrictions on which special characters can be used. A frequent restriction on special characters was ``do not use spaces". However, one piece of advice stated the more direct ``do not use special characters".

\paragraph{Don't repeat characters}
Not allowing the repetition of characters deters users from choosing passwords such as ``aaaaaaa" or ``wwddcc". Depending on the strictness of the restriction it could eliminate words such as ``bookkeeper" or ``goddessship". It could also cause some inconvenience for random password generators where the word ``Sdt2htTtd65c8h'' could be rejected.

\paragraph{Enforce restrictions on characters}
We collected twelve pieces of advice encouraging composition restrictions on passwords and only one piece of advice against it. The source rejecting composition rules was the NIST 2017 password guidelines. Abrams and Bulter find that password policies that require a minimum character length and mandate the use of specific character types may reduce the number of viable passwords by more than 60\% \cite{youtube_pwd_constraints}. Complex password composition rules can make the resulting passwords more difficult to guess \cite{kelley2012guess}. Though simply allowing only long (greater than 16 characters) passwords has a similar effect on guessability and may not cause as much hardship for users  \cite{kelley2012guess}. Both users and administrators indicated a number of minor costs associated with this advice. 
%%%%%%%%%%%%%%%%%%%%%%%%%%%%%%%%%%%%%%%%%%%%%%%%%%%%%%%

\subsection{Default Passwords}
Default passwords are used in IoT devices and WiFi equipment among other things. Manufacturers set  a default  password,  which  a user is supposed to change during setup \cite{farik2015analysis}. These default passwords are not secure as they have been shared publicly and often the same logins are used for many, or all, of the devices manufactured by a given company. Users marked the only cost as a need to create a new password. Though admittedly, we would see figuring out how to change the default password as another major time cost. Often administrator accounts exist on devices and have associated default passwords that the user of the device may know nothing about. 
All administrators surveyed agreed with changing default passwords.

%%%%%%%%%%%%%%%%%%%%%%%%%%%%%%%%%%%%%%%%%%%%%%%%%%%%%%%

%%%%%%%%%%%%% Expiry
\subsection{Expiry}
\paragraph{Store history to eliminate reuse }
This advice aims to stop users cycling through previously used passwords. Storing the history means there is an additional password file which needs to be protected. Because of the close relationship between old and new passwords \cite{zhang2010security}, if this file is revealed then the information
in it can be used to effectively guess the current password \cite{das2014tangled}. The organization must store all previous passwords, requiring memory resources. The user will need to pick a new password as old passwords cannot be reused. There is also an \textit{increased risk of forgetting} as the user may forget which passwords have been expired and which is the current password in use.

\paragraph{Change your password regularly}
From anecdotal evidence we know the advice ``change your password regularly'' is widely disliked by users \cite{hatechangingpass}. This is summarized by one user in our user study saying ``I hate this! The only solution I've come up with is to increment a number in the password each time. So inconvenient and frustrating, especially when combined with other bad password advice.''. 
%User survey 4 ID:624487-624478-66086963

Research has shown that the security benefits of expiry are minimal \cite{chiasson2015quantifying}\cite{zhang2010security} but still 7 organizations recommend the practice. This implies the inconvenience to users is worth less to organizations than the minimal security benefits. Or do organizations want to be seen to be enforcing strong security practices, and forcing expiry is just one way of doing this?

Only 50\% of the 40 end-users surveyed disagreed with regular password expiry. 25\% were neutral and 25\% agreed with it. For administrators we have a much smaller number of responses. However, 4 administrator respondents disagreed with expiry, 1 was neutral and 2 agreed.

\paragraph{Change if suspect compromise}
If there is a breach at the server the users were not at fault yet still they must choose a new password. The advice protects against online or offline guessing from an attacker who has access to the compromised password. All administrators and users approved of this advice.

%%%%%%%%%%%%%%%%%%%%%%%%%%%%%%%%%%%%%%%%%%%%%%%%%%%%%%%
%%%%%%%%%% Generated Passwords
\subsection{Generated Passwords}
The assumption by users for most of the advice related to generated passwords is that they will create their own password afterwards. This is evidenced by the inclusion of a costs for the user of creating a new password for most of the related advice. One user said ``Should also be replaced hence the added cost to create''. One issue an administrator flagged with generated passwords is that it is difficult to distribute them safely when off-site.

\paragraph{Use a random bit generator}
Random passwords are very difficult for users to remember \cite{zviran1993comparison} but passwords that aid memory retention can potentially lead to easier guessability.

\paragraph{Must aid memory retention}
Interestingly, the eight respondents who answered this question were split; 3 said it was a major cost and 3 said it was a positive cost. This is interesting as it depends on the interpretation. In comparison to choosing their own password, any generated password will be more difficult to remember. But in terms of a generated password that is randomly generated, it is easier to remember. We mark it as a minor\textit{ inconvenience to remembering a password} as the status quo of creating their own password would be easier to remember.

\paragraph{Must be issued immediately}
This decreases the chance that generated passwords are stolen before they are told to the user. If passwords were created in advance they would likely be recorded as administrators could not remember multiple generated passwords. This, therefore, protects against the potential for duplication while in storage.

\paragraph{Only valid for first login}
Because these generated passwords are often issued and created by administrators the user has no confidence in the security of their password up until the point they receive it. This advice protects against previous duplication of the password.

\paragraph{Distribute in a sealed envelope} 
Respondents to the user survey disagreed with whether this advice \textit{required extra resources}. Two said does not apply, two said minor and two said major. We suspect that though the organization may need the extra resources of envelopes, the end-users shouldn't need any extra resources. 
%%%%%%%%%%%%%%%%%%%%%%%%%%%%%%%%%%%%%%%%%%%%%%%%%%%%%%%

%%%%%%%%%%%% Individual Accounts
\subsection{Individual Accounts}
\paragraph{One account per user}
Having one account per user with a password is important for maintaining access controls and also tracking errors or attacks back to a source account. This will require organization time to set up. The cost can be high in an environment where there are shared computers. However, in our user study the majority of users assigned no cost to this piece of advice.  The alternative is multiple users using the one account. Compromises are more likely if there are multiple points of access. 

\paragraph{Each account password protected}
If there is no password we can likely consider the account to already be in a state of compromise. Password protecting an account increases the security of the account by necessitating one of the attacks to take place before an attacker can gain access.
User study respondents assigned very few costs to this advice. Surprisingly, half respondents said that \textit{need to create a new password} was a non-applicable cost. This could be because, even though a new password needs to be set, they don't necessarily need to create a new one as potentially an existing password could be used. However, we mark it as minor as it does require a new password to be set. 
The majority of administrators said there was no cost for implementation. We expect this is because it is considered standard on most systems. In fact, one administrators commented to say ``I haven't awarded severity/frequency costs because this should be mandatory and the cost is unimportant''.

%%%%%%%%%%%%%% Input
\subsection{Input}
\paragraph{Don't performed truncation}
One organisation advised that truncation of the password should never be enforced. That is, if a user creates a 12 character password, the verifier should not decide to just  store and compare the first 6 characters for authentication. Truncating passwords makes online and offline guessing easier. It can also affect social engineering attacks. If the user does not know that the password will be truncated they may reveal the first few characters of the password without realizing the true security risk of this action. The magnitude of the costs of not allowing truncation seem small though one administrator in our user survey did flag that truncation allows ``compatibility with legacy systems''.

\paragraph{Accept all ASCII characters}
One organisation argued for acceptance of all ASCII and UNICODE characters. This is expensive because it requires string normalization. The other organisation encouraged the removal of certain characters, specifically they recommended removing consecutive or all space characters. Accepting all characters reduces the likelihood that the policy will inconvenience a user's password choice. This increases the necessary search space of an attacker attempting online or offline guessing. Allowing all characters could give more scope for a SQL injection attack, but the hope is that there would be adequate string escaping in place to mitigate this. Administrators were asked about the costs of accepting all ASCII characters.

%%%%%%%%%%%%%%%%%%%%%%%%%%%%%%%%%%%%%%%%%%%%%%%%%%%%%%%

\subsection{Keep accounts safe}
\paragraph{Implement Defense in Depth}
This is a vague piece of advice, we do not know exactly what strategies would be deployed so we cannot fully capture the costs and benefits. One administrator said ``Its context specific based on the burden of costs associated with it''. It has the potential to mitigate any of the eleven attack types, but without knowing what is implemented we cannot say exactly what the security advantages or disadvantages are. 

\paragraph{Implement Technical Defenses}
The same argument as above can be used for this advice; it is not specific enough for us to know it's benefits. Though it is unlikely to aid against physical theft and social engineering. One respondent said that it is ``not specific or meaningful enough to be useful advice''.

\paragraph{Apply access control systems}
This means that only the privileged administrators have the power to view and control the authentication procedures and modify the stored authentication data. This protects against a malicious employee. Specific to authentication it can limit a malicious users' ability to change permissions, duplicating stored password data or downloading malware to attempt side channel or keylogging attacks. It can also protect against accidental damage by users. 
Access control can cause problems for end-users. One user survey respondent noted that ``The problem is that someone has to decide which parts of the system are relevant for everyone else, and it's easy to err on the `safe' side, which can create lots of friction.''

\paragraph{Monitor and analyze intrusions}
One respondent mentions that in order to follow this advice it is ``Assuming you know the attack vector''. This could mean working with users of the system and also engaging in user education so that users can recognise compromises. Computing power is also important for identifying and monitoring and analysing breaches. It is a major organisation cost to implement. 
This advice has no direct security affect unless the analysis is acted on.

\paragraph{Regularly apply security patches}
In order for security patches to be applied across an organisation, users must be compliant. Administrator survey respondents mentioned the difficultly of this task. One said that it ``requires a lot of additional management to be done properly and audited''. Another respondent mentioned that some patches can break existing functionality and a third emphasised that it is a big but necessary job.  Different security patches will protect against different attack types. 
%%%%%%%%%%%%%%%%%%%%%%%%%%%%%%%%%%%%%%%%%%%%%%%%%%%%%%%

%Keep your account safe
\subsection{Keep your account safe}
\paragraph{Check webpages for TLS}
This task helps users verify that communications to this webpage will be transmitted securely with encryption. This will help to combat phishing and pharming since phishing and pharming sites usually do not use SSL encryption. However, Dhamija et al. found that 23\%  of  their  participants  did  not  look  at  browser-based cues  such  as  the  address  bar,  status  bar  or  security indicators \cite{dhamija2006phishing} and Schechter et al found that 53\% of their study participants attempted to log into a site after they received a strong security warning \cite{schechter2007emperor}. This advice is not enforceable.

\paragraph{Manually type URLs}
Manually typing URLs can save a user from a Phishing attack as the user should recognize that the URL is not linking to the correct website. However, manually typing URLs makes a user vulnerable to typo-squatting/URL hijacking \cite{szurdi2014long}. A site with a similar URL, e.g. \url{www.goggle.com}, masquerades as the website of the user's intended destination and can trick a user into revealing their login details. Manually typing URLs can be very time consuming for users. 

\paragraph{Don't open emails from strangers}
In certain jobs it can be impossible to not open email from strangers and even in everyday life it can be very inconvenient. 
However, a 2012 study by B{\"o}hme and Moore found that as a result of concerns over cyber crime 42\% of participants say they do not open email from strangers \cite{bohme2012consumers}. We only collected one piece of advice which said not to open emails from strangers.

\paragraph{Keep software updated}
Vaniea and Rashidi found that 49.3\% of respondents relayed negative experiences with software updates. Keeping software updated protects against known security vulnerabilities. This can save a user from eavesdropping attacks, side channel attacks and endpoint compromise.  

\paragraph{Keep antivirus updated} 
Keeping antivirus updated is a periodic process for the user. It has the added disadvantage that the antivirus may also need to be repurchased regularly. Antivirus protected the user's machine from compromise.

\paragraph{Log out of public computers}
Not logging out of a public computer can lead to a lot of damage. An opportunistic attacker could spend money with linked credit cards, masquerade as the user, ask for money to be transferred by the user's peers, and set up backdoor access into the account for future use, among other things. We could find little evidence of reported breaches. It is unclear whether this is because it does not occur or whether victims don't reveal or don't know that this as the reason for their breach.

\paragraph{Password protect your phone}
Nowadays users can conduct most online transactions via mobile phones. Their portability makes them susceptible to theft. Also users are more likely to leave themselves continuously logged on to applications. Password protecting your phone reduces the chance of endpoint compromise. 
%%%%%%%%%%%%%%%%%%%%%%%%%%%%%%%%%%%%%%%%%%%%%%%%%%%%%%%

%%%%%%%%%% Length                                                                                                                         
\subsection{Length}
\paragraph{Enforce a minimum password length}
Enforcing a minimum length inconveniences memorability and may force users to alter or change their password. If our aim is to minimize password reuse, then this might not necessarily be a draw back \cite{herley2009so}. A minimum length will restrict the use of zero or one character passwords. Most of the advice encouraged the minimum length to be set at eight characters, likely as a protection against GPU-based guessing.

\paragraph{Enforce maximum password length}
Three pieces of advice recommended enforcing a maximum password length: 15 characters \cite{intel}, 20 characters \cite{paypal} and 40 characters \cite{interactivebrokers}. Interestingly, one company \cite{paypal} did not list a maximum password strength as one of their restrictions. Only when a user attempts to enter their password is the restriction revealed. NIST 2017 guidelines \cite{nist2017} state that  ``Verifiers should permit subscriber-chosen memorized secrets at least 64 characters in length". Restricting the length of a password inconveniences personal systems for password generation, restricts the outputs of a random password generator, and introduces an upper bound on the attacker's search space. It also makes passwords easier for an eavesdropper to record as they are less likely to cross packet boundaries.

%%%%%%%%%%%%%%%%%%%%%%%%%%%%%%%%%%%%%%%%%%%%%%%%%%%%%%%
%%%%%%%%%%%%%%%%%%%%%%%%%%% Multi factor authentication
\subsection{Multi-factor authentication}
\paragraph{Use multi-factor authentication}
Multi-factor authentication traditionally involves: \textit{something you are}, \textit{something you know}, and \textit{something you have}, e.g., fingerprint, password and a USB key token respectively. Using \textit{something you have} means that the user or organization may need to purchase an \textit{additional resource} and the user may need to carry an additional item. In addition, this item (unlike \textit{something you know} or \textit{something you are}) is susceptible to theft and loss. Though, if theft does occur the user is still nearly as secure as if the second factor had never been used. \textit{Additional user time} is needed to complete the authentication process since multiple factors are needed at each login. Using multi-factor authentication can decrease the success of phishing (as second factors are often not subject to replay) and online guessing attacks (as both factors must be guessed).

\paragraph{Use 2 step verification on phone}
Two step verification is different to multi-factor authentication as the two steps could use the same factor. 
Phones can be stolen or the code sent to the phone can be revealed by eavesdropping or a side channel attack. However if this occurs, depending on the chosen second step, the users' account could still be secure.

\paragraph{Use for remote accounts}
Remote accounts are often more vulnerable as the user might need to connect over an insecure channel. Depending on what the second factor is, physical theft or endpoint compromise could jeopardize the authentication. The probability the exchange is eavesdropped is much higher if used for remote accounts.
%%%%%%%%%%%%%%%%%%%%%%%%%%%%%%%%%%%%%%%%%%%%%%%%%%%%%%%

%%%%%%%%%%%%%%%%%%%%%%%%%% Network: Community Strings
 \subsection{Network: Community Strings}
 A community string is a user ID or password that is sent along with an SNMP request \cite{hare2010simple}. A community string is a password for access to statistics within a device or router. Someone can access data from such devices if they know the correct community string. 
 
 \paragraph{Don't define as standard default}
The standard default for community strings is set by the vendor. Vendors can choose the same password for all their devices and can have defaults passwords as simple as `public' \cite{jiang2002multiple}. These defaults are generally easily guessed. The community strings allow an attacker to find out about a organization's network and potentially find access points.

 \paragraph{Different to login password.}
Often community strings are not encrypted. Because they are transmitted in cleartext they can be read by anyone. This is an issue if the password sent is reused for other applications. A new string will need to be created but they are stored in configuration files and do not need to be memorized. 
%%%%%%%%%%%%%%%%%%%%%%%%%%%%%%%%%%%%%%%%%%%%%%%%%%%%%%%

%%%%%%%%%%%%%%%%%%%%%%Password cracking
\subsection{Password auditing}
\paragraph{Attempt to crack passwords}
By requiring users to change their password if it is guessed by an administrator the hope is that a stronger password will then be chosen by the user. This is a common policy for organizations \cite{klein1990foiling}\cite{yan2001note}, yet only one piece of advice we collected recommended it. We speculate whether organizations are unwilling to openly admit and recommend this practice. The cracking must be repeated periodically by the organization, meaning the password may need to be changed periodically by users. 

%%%%%%%%%%%%%%%%%%%%%%%%%%%%%%%%%%%%%%%%%%%%%%%%%%%%%%%

%%%%%%%%%%%%%%%%%%%%%%%%%%%%%%%%%Password managers
\subsection{Password managers}
\paragraph{Use a password manager}
If we assume the norm is for users to memorize their passwords, then a password manager does not, in its own right, offer additional security. It does greatly reduce the users' memory load and by extension then a user can use as long, random and complex of a password as they wish. Thus this act will increase security but just using the password manager does not guarantee users will increase the complexity of their passwords. A password manager does mean that the user is relying on an external agent to store their passwords and therefore if this agent is compromised then the passwords of all accounts are compromised. Therefore, we consider this to be a new way in which the users' password can be duplicated. A password manager requires additional resources for the user as the user may need to purchase and/or download and maintain a password manager.

\paragraph{Create long random passwords}
One of the advantages of a password manager is that, because a user no longer needs to recall their passwords, the password can be as long and complex as a user wishes \cite{florencio2014password}. Creating long and random passwords takes computing time and the user may need to specially configure the password manager. An organization specifying the type of password that should be created will inconvenience the users' personal system for password generation. If the password created is different to the users' general structure and is random, the user may never be able to remember it. This is only an issue if the password manager fails, the master password is forgotten or the user needs to access the account from a device not linked to the password manager.
%%%%%%%%%%%%%%%%%%%%%%%%%%%%%%%%%%%%%%%%%%%%%%%%%%%%%%%

%%%%%%%%%%%%%%%% Personal Information
\subsection{Personal information}
\paragraph{Don’t include personal information}
This is a difficult thing for an organization to enforce. In fact, there is no reasonable way for an organization to eliminate all personal information from passwords. Some basic form of cross checking between user information could be done. For example, at the client end it could be possible to sweep the information on a device to ensure it is not included. Doing this has high organization and user end computing costs as well as privacy/GDPR implications. It also has the potential to inconvenience the users' personal system for password generation. There is also an \textit{Increased risk of forgetting} as personal details could have made the password more memorable. If the advice is followed it would protect against a targeted attack. Castelluccia et al., find they can crack 5\%\ more passwords by leveraging personal information about users \cite{castelluccia2013privacy} and Li et al. discover that just over 60\% of passwords in their study of a Chinese password dataset contain at least one piece of personal information \cite{li2017personal}.
 
 \paragraph{Must not match account details} 
An increase in computing power is needed to cross check the password against the user's information. The advice is enforceable and protects against elementary targeted attacks. A simple form of this are `Joe accounts' where the username and password match \cite{joeusers}. In 1989, Bishop and Klein cracked 40\% of 14,000 UNIX accounts using guesses derived from associated usernames or account numbers and dictionaries \cite{bishop1995improving}.

\paragraph{Do not include names}
We consider a ban on names to be capable of eliminating a significant number of options for users' passwords and may make them more difficult to remember. In addition, words which double as names could be eliminated, ``Bob", ``Amber", ``Jack", as a result of this restriction.
%%%%%%%%%%%%%%%%%%%%%%%%%%%%%%%%%%%%%%%%%%%%%%%%%%%%%%%

%%%%%%%%%%%%%%% Personal password storage
\subsection{Personal password storage}

\paragraph{Don't leave in plain sight}
If the users are internal to the organization then it could be possible for the organization to monitor work areas. However in many situations it will be impossible. If the user follows the advice they have two options. They can memorize the password in which case there is a chance it is forgotten. Or they can store it in a hidden location which will require extra user effort or time to retrieve. This cost will take effect at every login as the user will need to check the password each time. 

\paragraph{Don't store in a computer file}
 This advice is difficult or impossible for an organization to enforce. An attacker accessing the file can duplicate passwords.
 
\paragraph{Write down safely}
Even if the password is stored safely, the very act of writing it down makes it's duplication and physical theft possible. There is discussion as to whether the security risks of writing passwords are in fact very low \cite{schneierwritedown}. In fact, if users write down passwords then they may be more confident making stronger password choices \cite{cheswick2013rethinking}\cite{komanduri2011passwords}\cite{herley2009so}. Users will have to take the time to look-up the password when they need to enter it. Shay et al., find that users are more likely to share and reuse their passwords than write them down \cite{shay2010encountering}.

\paragraph{Don't choose ``remember me''}
If the ``remember me'' option is not used then if an attacker steals a laptop or computer they should not automatically have access to the accounts on it. It is equivalent to not logging out of an account. The user will now need to remember their password instead of it being saved in the browser. In additio,n at each login the user will need to physically type their password. 
%%%%%%%%%%%%%%%%%%%%%%%%%%%%%%%%%%%%%%%%%%%%%%%%%%%%%%%
%%%%%%%%%%%%% Phrases
\subsection{Phrases}
\paragraph{Blocklist common passwords \& Don't use patterns \& Don't use words \& Don't use published phrases}
Needing to Blocklist common words or remove all patterns during password creation could be computationally expensive for the organization if the list becomes very large.  There exists a PAM module called `cracklib' which automates blocklisting \cite{muffet1997cracklib}. From leaked password database we know users primarily choose words and pattern based passwords \cite{rockyou}. Shay et al. find that the ``use of dictionary words and names are still the most common strategies for creating passwords" \cite{shay2010encountering}. This depicts how ineffective some password advice can be and is possibly a reflection on the costs appearing to not outweigh the benefits from a users' point of view. 

\paragraph{Substitute symbols for letters}
We know from Warner \cite{subs} that passwords with simple character substitutions can be weak. Yet, 2 of 3 pieces of advice recommend it. This could stem from the attitude that it is `better than nothing'. 

\paragraph{Insert random numbers and symbols \& Take initials of a phrase}
Unless an organization automates password generation, it is difficult to enforce. Taking initials of a phrase can make a password appear like a random string.

\subsection{Policies}
\paragraph{Establish clear policies}
A lot of the advice we have collected is contradictory. Including the advice from the two organizations who gave this advice! This advice does not directly increase or decrease the probability of success of an attack type.
%%%%%%%%%%%%%%%%%%%%%%%%%%%%%%%%%%%%%%%%%%%%%%%%%%%%%%%

%%%%%%%%%%%%%%% Reuse
\subsection{Reuse}

\paragraph{Never reuse a password} 
Users must create a new password each time they open an account. It is very hard to enforce a no reuse policy across organizations. Das et al. estimate that 43-51\% of users reuse passwords across sites \cite{das2014tangled}. If passwords are reused then online and offline guessing becomes much easier for an attacker.

\paragraph{Don't reuse certain passwords}
Asking users to not reuse certain passwords is equivalent to saying that a user can reuse some passwords. Flor{\^e}ncio, Herley and Van Oorschot \cite{florencio2014password} declare that, ``password re-use is a necessary and sensible tool in managing a portfolio'' of credentials. They recommend grouping passwords according to their importance and reusing passwords only within those groups. If we look at the specific advice in this category, we see that most organizations are asking users to not reuse the password for \underline{their} site. This does provide some security advantage for that specific site. The attacker will not be able to directly access the protected account using a compromised password from another source. However, an attacker can leverage information from other compromised sites to attempt phishing, social engineering and guessing attacks with more success.
%could remove the flor cite & description

\paragraph{Alter and reuse passwords}
Das et al. \cite{das2014tangled} were able to guess approximately 10\% of non-identical password pairs in less than 10 attempts and approximately 30\% in less than 100 attempts. Therefore, we mark this as a limited security improvement. We could find no research suggesting this method of altering and reusing passwords as effective, though anecdotally it is common \cite{stobert2014password}. Specifying the structure that passwords should take could partially affect users' personal system for password generation. 

%%%%%%%%%%%%%%%%%%%%%%%%%%%%%%Sharing
\subsection{Sharing}
\paragraph{Never share your password \& Don't send passwords by email \& Don't give passwords over phone}
Weirich and Sasse find that sharing your password is regarded as a gesture of trust and refusing to share your password with someone is an indication that you do not trust them \cite{weirich2001persuasive}. A 2011 study of 122 people found that one third of respondents reported sharing their personal email password, a quarter shared their Facebook password and approximately 20\% of people who had work email passwords reported sharing them with colleagues \cite{kaye2011self}. However, Kaye finds that thought and consideration was given before the password was shared. This tells us that the user is aware of the security risks and may accept them on the ground of trust. In the process of sharing a password it could be eavesdropped. Not allowing users to share their passwords also helps to protect against social engineering, though this is through the form of user education.

%%%%%%%%%%%%%%%%%%%%%%%%%%%%%%Shoulder surfing
\subsection{Shoulder surfing}
\paragraph{Offer to display password}
A visual image of the passwords could help users with the memorization of their password or aid users with difficulty typing. Nielsen in 2009 challenged ever masking passwords \cite{nielsenmasking}. Bruce Schneier, after originally agreeing with the removal of masking, here \cite{schneiermasking} sums up why password masking needs to continue in certain contexts. 

\paragraph{Enter your password discretely}
This advice is unenforceable. But Flor{\^e}ncio, Herley and Coskun suspect that shoulder surfing attacks are not very common as humans are very good at detecting people in their personal space \cite{florencio2007strong}. Eiband et al. find that shoulder surfing mainly occurs in an opportunistic, non-malicious way and it is usually personal data that is observed \cite{eiband2017understanding}. When a user is logging in it may take some extra time or inconvenience for them to verify that they are entering their password discretely.

%%%%%%%%%%%%%%%%%%%%%%%%%storage
\subsection{Storage}
\paragraph{Encrypt passwords file}
This is the encryption, usually with a password as the key, of the file containing all the passwords. Encrypting this file means that when any user wishes to log in, the whole file is decrypted, the password is compared to the value entered by the user, and then the file is encrypted again. Encrypting the individual password values is different and is discussed below. Encryption and decryption  may slow down the authentication process for the user. For the organization, at each system start up the password needs to be provided. This can be done manually, which would require periodic organization time. Or it could be automated in which case the password is accessible to the computer system, which would bear security risks, by reducing the effective secrecy provided by the encryption.

\paragraph{Restrict access to password files}
The advice in this category recommended encrypting the file the passwords are stored in and restricting access to those files. An example of this in practice is Unix's /etc/shadow file versus the /etc/password file. Access controls are implemented in Unix and Linux machine and result in a secure out of the box authentication protocol.

\paragraph{Store password hashes}
A cryptographic hash is a bit string of a fixed size which should uniquely represent a password. It is irreversible but is deterministic i.e. the same password will always map to the same hash. An attacker can discover the passwords by creating a large look up table (rainbow tables) which matches each password to a corresponding hash value. This is very effective for passwords up to a certain length and after this point a brute force search is still possible. If the hash of the password is stored, then if the user forgets their password, the password cannot be recovered from the hash. Therefore the user will need to create a new password. 

Two pieces of advice recommending hashes also recommended using a salt. The salt randomizes the output of the password hash, making the use of rainbow tables impossible. An offline guessing attack is necessary for revealing the passwords. One piece of advice relating to salting said to use ``a unique salt for each account''. The second piece did not specify whether the same salt could be used for all accounts of whether a unique salt was to be used. If the same salt is used then a look up table is still a feasible attack. Not specifying the use of a salt might be a careless use of terminology, but a 2019 paper by Ntantogian et al. found that 14.29\% of Content Management Services surveyed did not use a salt in their default hashing scheme \cite{ntantogian2019evaluation}.

\paragraph{Encrypt passwords}
Encryption of passwords was the first common method recommended as a means of protecting passwords \cite{morris1979password}. However it is often reversible and a key needs to be protected for security to be maintained. It is now recommended that the hashing and salting method is used for password storage. Despite this, seven pieces of advice recommended password encryption, in comparison to only four pieces of advice recommending hashing and only two recommending hashing and salting. N

In the case of a password leak, either the key is revealed along with the password database or it is not. If the key is revealed all passwords are immediately decryptable. If the key is not revealed then brute force guessing can be attempted against the key, but this is a difficult task. In the adobe breach, for example, though most passwords were compromised by guessing the key was never discovered \cite{adobe_guardian}.

\paragraph{Don't hardcoding passwords}
Hardcoding passwords will make is very difficult to automate changes making it a less usable method. Hardcoding will also make passwords less secure since they may be stored in plaintext to a file that an administrator can directly edit.

%%%%%%%%%%%%%%%%%%%%%%%%%Throttling
\subsection{Throttling}
\paragraph{Throttle password guesses}
Throttling involves limiting the number of wrong guesses that can be made against an account. However, because of the right-skewed nature of password distribution, the attacker does still have a high probability of success with a small number of guesses \cite{malone2012investigating}\cite{murray2018exploring}. The cost of this is that a legitimate user could accidentally be locked out if they mistype or forget their password a certain number of times.  For example, Brostoff and Sasse \cite{brostoff2003ten} find that with a three strike system 31\% of users are unfairly locked out.

%%%%%%%%%%%%%%%%%%%%%%%%%%%%Transmitting passwords
\subsection{Transmitting passwords}
\paragraph{Don't transmit in cleartext \& Request over a protected channel}
These are very similar pieces of advice since both groupings place the onus on the organization to oversee that passwords are sent by protected channels. If passwords are transmitted in cleartext they are susceptible to any eavesdropper on the network. Let's Encrypt has helped to make security certificates accessible to more websites \cite{letsencrypt}. However providing a secure channel for passwords is not an easy task. In a 2017 2-hour lab study, 18.5\% of educated participants failed to set up a secure HTTPS connection \cite{krombholz2017have}.

%%%%%%%%%%%%%%%%%%%%%%%%%%%%Username
\subsection{Username}
\paragraph{Enforce composition restrictions on usernames}
Flor{\^e}ncio, Herley and Coskun argue that it is better to increase the strength of the userID rather than the passwords \cite{florencio2007strong}. They propose that this will protect against online guessing attacks but will not majorly increase the cost to users since the username can be recorded visibly.

\paragraph{Don't reuse username}
If the same username is used for multiple accounts then once the password for one account is compromised, this password can be tried against the same person's other accounts. Das et al. find that 43-51\%,  of  users  directly  re-use  passwords between  sites and many others introduce small modifications to their passwords across sites \cite{das2014tangled}. Not reusing a username could be one way to protect against an attacker leveraging this vulnerability and could be less burdensome on the user than a restriction on altering and reusing passwords. However, many sites require an email address as a username and it is not reasonable to prohibit reuse of an email address. 

\subsection{Don't allow users to paste passwords}
We manually added this advice to our collection because, though we did not collect it, there is a tradition of not allowing users to paste passwords. There is no clear evidence for the origin of this advice and users often questions why they are not allowed to paste their passwords into the password field  \cite{troypaste}. This advice has 4 different costs: the organization must implement it, the user must take the extra time to manually type the password, many password managers cannot function without pasting, users are at a much higher risk of typos, and a user may need to choose a much shorter password if they cannot simply paste it efficiently into the web-form at login. Also, often the user has already created their password before this rule is revealed. There appears to be no security benefits to this advice \cite{sachapaste} and indeed in our model we cannot find any attack type that it mitigates.
