# Supplementary material for: Costs and benefits of authentication advice
Source: arXiv:2008.05836 source file (2023-02-16)
Supplement: Supplementary file 4 [file org_adv_exp.tex]

%%%%%%%%%%%%%%%%%%%%%%%%%%%%%%%%%%%%%%%%%%%%%%%%%%%%%%%%%%%%%%%%%%%%%%%%%%%

%\subsubsection{Access to password file}

\subsubsection{Administrator Accounts}

\paragraph{Not for everyday use}
 The main cost here is to the administrator who must switch between accounts for different tasks. Though this burden is lessened by the implementation of programs such as su and sudo which allow users to easily run programs which require extra security privileges. In the time constraint we consider the administrator to be a user. The organization must also have the resources to create two accounts for the one user. 

\paragraph{Must have its own password}
This requires the organization to set up password protection on the administrator account. The administrator must create a new password and enter it in some way at each login. Multiple users with privileged access may all need to know the same administrator password. This is the disadvantage of using su protocols over sudo. 

\paragraph{Should have extra protection}
This advice is so vague that it is impossible for us to determine what exact costs are associated with it. We can assume that the organization will need to set these extra protections in place. It is likely to take time for the user, but with out knowing what the protections are we cannot say. Both sudo and su provide additional protection for administrator accounts.

\subsubsection{Default passwords}
\paragraph{Change all default passwords}
This requires changing from default passwords but does not require that each password is unique and they often may be recorded, thus not requiring much additional burden on users. The most inconvenient aspect would be identifying all the default passwords that are in use the technology used by the organization. Often administrator accounts exist on devices and have associated default passwords that the user of the device may know nothing about.

\subsubsection{Expiry}
\paragraph{Store history to eliminate reuse }
The organization must store all previous passwords, requiring memory. The user will need to pick a new password as old passwords cannot be reused. At creation the server must query the stored dataset to verify the uniqueness of the new password. There is also an \textit{Increased risk of forgetting} as the user may forget which passwords have been expired and which is the current password in use.

\paragraph{Change your password regularly}
Organizations will need to notify users of the requirement to change their password. The organization will need to update their stored dataset of passwords at each update. 
Because passwords regularly need to be changed we anticipate an increase in the memory load over time. Users will repeatedly \textit{need to choose a new password}. On top of this will be an \textit{increased risk of forgetting} as a result of the repeated changes. 

\paragraph{Change if suspect compromise}
The advice under this statement was ambiguous as to whether it was being aimed at a user or at an organization. We have chosen to interpret it as if it is aimed towards an organization. In this way the statement tells an organization that if they become aware of a compromise they should ensure that their users' passwords are changed. This is the correct interpretation for five of the ten pieces of advice in the category. It is also a more interesting way to interpret advice as the advice aimed at the user is unenforceable. 

An organization can either internally monitor breaches or link with a breach application. For example receiving notifications about their users' credentials from \url{https://haveibeenpwned.com} \cite{haveibeenpwned}. The notifications to users then will require organization time and updating password files will require computing power.

\subsubsection{Generated passwords}
\paragraph{Must be issued immediately}
Uses users time as the user must be available to receive the newly created password. Takes administrator time to distribute.

\paragraph{Only valid for first login}
Requires the user to generate their own password as well as administrators to generate the initial generated password. 

\subsubsection{Individual accounts}
\paragraph{One account per user}
This will require organization time to set up and resources to provide server space for the account. Different users using the same device will need to switch between their accounts, this logging in and out will cost the organization computing power and the user time.

\subsubsection{Input}
\paragraph{Don't performed truncation}
There will be an increase in computing power for hashing the additional characters and the user must now enter their entire password correctly each time. As a comparison also see the costs and benefits assosiated with setting a maximum password length.

\paragraph{Accept all characters}
The organization must create a system which has the ability to accept all characters in a consistent way. This is a non trivial task. It will involve the standardization of Unicode characters entered from any keyboard at each login. Accepting all characters reduces the likelihood that the policy will inconvenience a user's password choice.

\subsubsection{Keep accounts safe}
\paragraph{Implement Defense in Depth}
Because we do not know what defense in depth strategies would be deployed, we cannot fully capture the costs. We can say that the defense in depth will require organizational time to put in place.

\subsubsection{Length}
\paragraph{Minimum password length}
This advice \textit{increases the risk of forgetting} simply because the user needs to remember more characters. It also \textit{inconveniences  the users' personal system for password generation} as a user may not be able to use a password within their normal structure. 

\paragraph{Enforce maximum length (\textless40) }
This advice \textit{inconveniences  the users' personal system for password generation} as a user may wish to choose a longer password. In fact one of the pieces of advice we collected, told the organization to limit the password length to less than 15 characters. This inconvenience will also increase the chance that the user forgets the password. There is no additional reason for this advice to hinder memory and therefore \textit{increased risk of forgetting} is not marked in it's own right. 

Enforcing a maximum length saves on encrypting and sending a very long password. This would be a reduction in computing time. But needing to check the length requires a very small increase in the computing time. We say that these cancel out and any overall impact this advice has on the computing power is small.

\subsubsection{Network: Community strings}
\paragraph{Different to login password}
The user needs to create a new password. The community strings are often stored in configuration files and do not need to be memorized by the user.

\subsubsection{Shoulder surfing}
\paragraph{Offer to display password}
A visual image of the passwords could help users with the memorization of their password or users with difficulty typing. Therefore this advice has a positive effect on memorability and user inconvenience.

\paragraph{Enter your password discretely}
When a user is logging in it may take some extra time or inconvenience for them to verify that they are entering their password discretely.

\subsubsection{Storage}
\paragraph{Encrypt password files}
Encryption and decryption  may slow down the authentication process for the user. For the organization, at each system start up the password needs to be provided. This can be done manually, which would require periodic organization time. Or it could be automated in which case the password is accessible to the computer system, which would bear security risks, by reducing the effective secrecy provided by the encryption.

\paragraph{Store password hashes}
If the hash of the password is stored, then if the user forgets their password, the password cannot be recovered from the hash. Therefore the user will need to create a new password.

\subsubsection{Throttling}

\paragraph{Throttle password guesses}
Throttling involves limiting the number of wrong guesses that can be made against an account. The cost of this is that a legitimate user could accidentally be locked out if they mistype or forget their password a certain number of times.  For example, Brostoff and Sasse \cite{brostoff2003ten} find that with a three  strike system  31\% of users are unfairly locked out is.  With ten strikes it is 7\%. Smart systems can help to minimize the risk for real users \cite{microsoft_sync}.

\subsubsection{Don't allow users to paste passwords}
This advice has 4 different costs: the organization must implement it, the user must take the extra time to manually type the password, many password managers cannot function without pasting, users are at a much higher risk of typos, and a user may need to choose a much shorter password if they cannot simply paste it efficiently into the web-form at login. Also, often the user has already created their password before this rule is revealed.
