# Supplementary material for: Costs and benefits of authentication advice
Source: arXiv:2008.05836 source file (2023-02-16)
Supplement: Supplementary file 5 [file org_discuss_benefits.tex]

\subsubsection{Access to password file}
\paragraph{Encrypt password files}
Encrypting password files will protect against the theft of the hard drive. However, the password used for encryption could still be read from the RAM. If the system can access the password without manual intervention then the password is likely to be stolen if the encrypted file is stolen. An attacker will have more difficulty downloading the password file for offline guessing. 

\paragraph{Restrict access to password files}
Restricting access to password files will protect against certain types of unauthorized binding. If an attacker does not have access to the stored authentication details then the attacker will find it difficult to change the password stored for the user or link additional passwords or authenticators to the account. Preventing read access to a password file could prevent offline guessing attacks. 

\subsubsection{Administrator accounts}
\paragraph{Not for everyday use}
It can be argued that the more times the authentication process is completed by the user, the more times it is susceptible to compromise during entry or transmission. 
We therefore say that not logging into the administrator account for everyday tasks decreases the chance of eavesdropping and side channel attacks.

\paragraph{Must have its own password}
If there is one administrator then ensuring that this administrator account has a distinct password means it is less vulnerable to eavesdropping and side channel attacks. However in most situations, many users will require privileged administrator access. In this case the problem depends on how you choose to implement this advice. If users access the administrator privileges by typing the administrator password via su then all privileged users must know the same password. This makes social engineering, phishing and endpoint compromise more likely.  In addition if multiple users are recording or sharing with others the same credentials then they are more likely to be duplicated and fall into the hands of an attacker. 

Alternatively, there might be administrative access via the user's own password (e.g. via sudo) or a second administrative account/password corresponding to each user with administrative privileges. 

All of these have associated security risks. In our table we have represented the case where there is one administrator who must create a second password which allows them access to administrator privileges. 

\paragraph{Should have extra protection}
Depending on the extra protection the account is given this will have different benefits.

\subsubsection{Backup work}
\paragraph{Make digital \&\ physical back-ups}
Having a back up of work means that attacks can be less harmful to the organization. Having backups does not directly decrease the chance of an attack but would be factored in in relation to the costs of a breach. Having physical backups of work does mean that the potential for physical theft now exists.

\subsubsection{Expiry}
\paragraph{Store History to eliminate reuse}
This advice is given alongside ``Change your password regularly''. The password must now also not match any previous passwords. This means that knowledge of old passwords will not directly lead to an attacker knowing a current password.

However, even though users can no longer reuse prior passwords, alterations are still possible \cite{shay2010encountering}. In fact, Zhang, Monrose and Reiter \cite{zhang2010security} identify that we can easily predict new passwords from old when password aging policies force updates.

In addition, if an attacker gains access to a users' account and changes their password, the user will be unable to change it again until the required number of days have elapsed, or with an administrator's help.

Finally, storing the history means there is an additional password file which needs to be protected. Because of the close relationship between old and new passwords \cite{zhang2010security}, if this file is revealed then the information
in it can be used to effectively guess the current password \cite{das2014tangled}.  

\paragraph{Change your password regularly}
In a certain situation changing your password regularly does decrease the probability of success of online guessing. Imagine an attacker cycling through a list of guesses. If a password is changed to something new during this guessing, then an attacker wishing to guess it must start their guessing process again from scratch. 

However, most attackers will guess the most probable guesses first and since passwords follow a long tailed distribution \cite{murray2018exploring,malone2012investigating} a rational attacker will typically stop and move onto a new account if the password is not captured within the first few million guesses. 

If the attacker correctly guesses the password within the time frame. Then the password will be changed at the beginning of the new period. This does bring some additional security but in reality once an attacker has access to the account they can set up a backdoor and will not need the password in future. Even if the attacker creates no backdoor the probability that they can guess the next period's password is high as users base their next password heavily on their previous password \cite{zhang2010security,das2014tangled}. Therefore, knowledge of the password from one period will strongly aid the attacker in guessing subsequent passwords.

\paragraph{Change if suspect compromise}
If the password has been leaked elsewhere then the advice is to change your password. This protects you from online or offline guessing attacks as otherwise an attacker with access to compromised password has immediate access to the account. Some of the caveats discussed above still apply. But the hope is that if a compromise is suspected, a user may be less likely to create a new password very similar to their old one. In addition the time scale to the creation of backdoor may be longer.

\subsubsection{Generated passwords}
\paragraph{Must be issued immediately}
This decreases the chance that generated passwords are stolen before they are told to the user. If passwords were created in advance they would likely be recorded as administrators could not remember multiple generated passwords. Therefore these passwords could be duplicated while in storage.

\paragraph{Distribute in a sealed envelope} 
This increases the chance that the password is physically stolen as the envelope could be taken. The password could also be duplicated since it has been recorded. If an adversary opens the envelope and duplicates the password then it will go undiscovered if the adversary places the password page in a new envelope and reseals it. The benefit of the sealed envelope is that an observational, audible or network eavesdropping attack is less likely. 

\paragraph{Only valid for first login} 
Because these generated passwords are often issued and created by administrators the user has no confidence in the security of their password up until the point they receive it. Maintaining a rule that passwords must be changed at first login means that the user can now have complete control over the security of this new password. This advice then protects against previous duplication of the password.

\subsubsection{Individual accounts}
\paragraph{One account per user}
The alternative is multiple users using the one account. With multiple users using the same account one user could modify the authentication information without informing other users (unauthorized binding). In addition, if multiple users are recording or sharing with others the same credentials, then they are more likely to be duplicated and fall into the hands of an attacker. Social engineering and phishing attacks and endpoint compromise are also more likely if there are multiple points of access.

\paragraph{Each account password protected}
If there is no password we can likely consider the account to already be in a state of compromise. Password protecting an account increases the security of the account by necessitating one of the attacks to take place before an attacker can gain access. It obviously protects against both online and offline guessing. In addition having a password makes a side channel attack more complex. An attacker should be able to differentiate the difference between an account login where no password is used and when a password is used.
%not end pt com
%not physical theft
%offline guessing -yes DING{58}
%side channel - sending no password looks different from sending a password. potentially \down
%online guessing - yesDING{58}
%

\subsubsection{Input}
\paragraph{Don't performed truncation}
Truncating passwords makes online and offline guessing easier. It can also affect social engineering attacks. If the user does not know that the password will be truncated they may reveal the first few characters of the password without realizing the true security extent of this action. 

\paragraph{Accept all characters}
This increases the necessary search space of an attacker attempting online or offline guessing. Allowing all characters could give more scope for a SQL injection attack, but the hope is that there would be adequate string escaping in place to mitigate this fear. We account for the implementation difficulties in costs.

\subsubsection{Keep accounts safe}
\paragraph{Implement Defense in Depth}
Defense in depth can be divided into three categories: physical controls, technical controls and administrative controls. The security defense in depth can provide depends on exactly what strategies are deployed. They have the potential to mitigate any of the eleven attack types but without knowing what is implemented we cannot say exactly what the security advantages or disadvantages are.

\paragraph{Implement Technical Defenses}
The same argument as above can be used for this advice; it is not specific enough for us to know it's benefits. Though it is unlikely to aid against physical theft and social engineering. 

\paragraph{Apply access control systems}
Access controls make sure that only certain users have access to their required aspects of the system. With respect to authentication, this means that only the privileged administrators have the power to view and control the authentication procedures and modify the stored authentication data. This protects against a malicious employee ``turning off'' authentication or other security mechanics, duplicating the stored password dataset or downloading malware to attempt side channel or keylogging attacks. However, exactly what this advice protects against depends on which specific access controls are put in place. 

\paragraph{Monitor and analyze intrusions}
Awareness of what an attacker is doing within the system and learning where the vulnerability is is important for security. However this advice has no direct security affect unless the analysis is acted on. For example, if an administrator witnesses an attacker duplicating the plaintext password file, then a forced password change might need to be implemented. Else if an administrator witness an attacker binding an additional form of authentication to a user or changing the credentials for a user, then these actions would need to be reversed. Monitoring and analyzing intrusions could also guide user education. 

%\paragraph{Regularly apply security patches}%aaa

\subsubsection{Length}
\paragraph{Minimum password length}
Inhibits brute force guessing as there are no passwords to guess with a very small number of characters, which are sometimes favoured by both users and guessers. 

\paragraph{Enforce maximum length (\textless40)}
Requiring that passwords are less than a certain number of characters makes them easier for an eavesdropper to record them as they are less likely to cross packet boundaries. It also makes online and offline guessing easier as the attacker now need only guess passwords within the given range. 

\subsubsection{Policies}
\paragraph{Establish clear policies}
This advice does not directly increasing or decrease the probability of success of an attack type.  

\subsubsection{Throttling}
Throttling (or rate limiting) password guesses drastically reduces the number of guesses an attacker can make. The attacker can no longer continuously make guesses until the correct password is accepted. However, because of the right-skewed nature of password distribution, the attacker does still have a high probability of success with a small number of guesses \cite{malone2012investigating}\cite{murray2018exploring}.

\subsubsection{Don't allow users to paste passwords}
There appears to be no security benefits to this advice \cite{sachapaste} and indeed in our model we cannot find any attack type that it mitigates.
