# Supplementary material for: Costs and benefits of authentication advice
Source: arXiv:2008.05836 source file (2023-02-16)
Supplement: Supplementary file 6 [file user_adv_exp.tex]

\subsubsection{Backup password options}
\paragraph{Email up-to-date and secure}
Most organization can not practically check that each user has kept their email up-to-date and secure. For a compliant user, this is a continuous process and will cost the user their time.

\paragraph{Security answers difficult to guess}
It is unlikely an organization will be able to enforce this advice. One option could be to employ guessing and require users to change their answers if they have been guessed. But in reality a practice such as this would have its own additional costs associated with it. Security answers which are difficult to guess will likely be difficult to remember and will also take time for the user to create. 

\paragraph{Do not store hints}
This statement represents two pieces of advice. One of the pieces of advice tells organizations to not allow users to store a hint, and one tells a user to not store a hint. 
An organization is unlikely to be able to stop users from storing password hints. However they can opt to not provide the facility for it.
We look at the costs from the point of view of the advice aimed at the user, i.e. the user voluntarily following the advice to not store a  hint.

\subsubsection{Composition}
For all three advice statements in this category the same costs are identified. The organization uses small amounts of computing power to verify that the password meets the requirements. 

\paragraph{Don't repeat characters}
Not allowing the repetition of characters deters users from choosing passwords such as ``aaaaaaa'' or ``wwddcc''. Depending on the strictness of the restriction it could eliminate words such as ``bookkeeper'' or ``goddessship''. It could also cause some inconvenience for random password generators where the word ``Sdt2htTtd65c8h'' could be rejected.

\subsubsection{Keep your account safe}
All the advice in this category requires user time. ``Check web pages for SSL'', ``Manually type URLs'' and ``Don't open emails from strangers'' are marked as periodic as they need to be repeated regularly. 
Both ``Keep anti-virus updated'' and ``Keep software updated'' require \textit{additional computing power}. The \textit{additional resource} of anti-virus software is definitely needed for the former and it is possible additional resources are also needed for the latter. 
Both ``Log out of public computers'' and ``Password protect your phone'' have the potential to introduce an increased password memory burden on users. 

The organization does not have the ability to enforce most of this advice. We mark it as voluntary for the users to follow. Alternatively, we could introduce organization time costs for the time spent on user education.

\subsubsection{Multi-factor authentication}
\paragraph{Use multi-factor authentication}
It is likely that either the user or the organization will have to provide the \textit{additional resource needed }for authentication, for example a USB token. We underline this cost as it depends on the implementation whether it is the user or the organization who must purchase the additional resources. 

\textit{Additional user time} is needed to complete the authentication process since multiple factors are needed at each login. Some devices do offer a ``remember me on this device option'' which would ease the burden on the users. But this will have it's own security trade-offs.  

Multi-factor authentication will require \textit{additional computing power} for both the user and the organization to authenticate someone with multiple factors.
If the user is using `something you have' to authenticate and loses it, this will also have an impact for \textit{user time and inconvenience}. Also, the user must remember to bring the device with them.

\paragraph{Use for remote accounts}
The costs for this piece of advice are similar to those for ``Use multi-factor authentication''. The difference is that the costs only need to apply to remote accounts. It does require the same amount of organization time to implement.

\subsubsection{Password managers}
\paragraph{Use a password manager}
A password manager helps a user by remembering their passwords and saves the user the time of typing the password at each site. A password manager will use some computing power. Some organizations will be able to force all their users to use a password manger but most organizations will not have this capability. This requires additional resources for the user as the user may need to purchase and/or download and maintain a password manager.

\paragraph{Create long random passwords when using a password manager}
One of the advantages of a password manager is that, because a user no longer needs to recall their passwords, the password can be as long and complex as a user wishes. Creating long and random passwords takes computing time and the user may need to specially configure the password manager. An organization specifying the type of password that should be created will inconvenience the users' personal system for password generation. If the password created is different to the users' general structure and is random, the user may never be able to remember it. This is only an issue if the password manager fails, the master password is forgotten or the user needs to access the account from a device not linked to the password manager.

\subsubsection{Personal Information}
\paragraph{Don’t include personal information}
This is a difficult thing for an organization to enforce. In fact, there is no reasonable way for an organization to eliminate all personal information from passwords. Some basic form of cross checking between user information could be done. For example, at the client end it could be possible to sweep the information on a device to ensure it is not included. Doing this has high organization and user end computing costs as well as privacy/GDPR implications. It also has the potential to inconvenience the users' personal system for password generation. There is also an \textit{Increased risk of forgetting} as personal details could have made the password more memorable. 

\paragraph{Must not match account details} 
An increase in computing power is needed to enforce this as the password needs to be cross checked against the user's information.

\paragraph{Do not include names}
We consider a ban on names to be capable of eliminating a significant number of options for users' passwords. This can \textit{Inconveniences users' personal system for password generation} and make passwords more difficult to remember.

\subsubsection{Personal Password Storage}
\paragraph{Don't leave in plain sight}
If the users are internal to the organization and work areas are monitored then it could be possible for an organization to enforce this advice. However in many situations it will be impossible. If the user follows the advice they have two options. They can memorize the password in which case there is a chance it is forgotten. Or they can store it in a hidden location which will require extra user effort or time to retrieve. This cost will take effect at every login as the user will need to check the password each time. 

\paragraph{Write down safely}
Encouraging users to write their password down means they are less likely to forget it. Therefore this is a positive for the cost category \textit{Increased risk of forgetting}. It is not particularly enforceable by the organization and will require user time to record the password and check it at each login. 

\paragraph{Don't choose ``remember me''}
The user will now need to remember their password instead of it being saved in the browser. In addition at each login the user will need to physically type their password.

\subsubsection{Phrases}
Needing to Blacklist common words or remove all patterns during password creation could be computationally expensive for the organization if the list becomes very large.  There exists a PAM module called `cracklib' which automates blacklisting \cite{muffet1997cracklib}.

``Take initials of a phrase'' and ``Substitute symbols for letters'' are both impossible to enforce. Unless an organization automates password generation, it is difficult to enforce ``Insert random numbers and symbols''. If it was automated it would carry little to no security benefits since it would be a known procedure.

\subsubsection{Reuse}
\paragraph{Never reuse a password} 
If users never reuse a password they must create a new password when they open the account. Because we are looking at a snapshot for a particular organization we assume users will have just one account in the lifetime. Therefore we do not mark this as having repeating costs though from a users' perspective it does. 

Password reuse could be within an organization or across organizations. It is very hard to enforce a no reuse policy across organizations. 

\paragraph{Alter and reuse passwords}
Specifying the structure that passwords should take could partially affect users' personal system for password generation.

\subsubsection{Username}
\paragraph{Enforce restrictions on characters}
We mark this as requiring the cost \textit{Inconveniences users' personal system for password generation}. While it is not a password, the advice does inconvenience the users' personal system for generating a username and, as such, could have similar costs.
