# Supplementary material for: Costs and benefits of authentication advice
Source: arXiv:2008.05836 source file (2023-02-16)
Supplement: Supplementary file 7 [file user_discuss_benefits.tex]

\subsubsection{Back up password options}
\paragraph{Email up-to-date and secure. }
Email is used for password reset links and often as the method that a generated password is passed to users. Therefore having a secure email account can help against eavesdropping of passwords by attackers. It can also prevent unauthorized binding of a new password to a users' account through the form of an emailed password reset. Having an up-to-date and secure email system with a working spam/malware filter can help to protect against phishing and pharming attacks and compromise of an endpoint due to malware.

\paragraph{Do not store hints}
If hints were stolen then these hints could be used to facilitate online or offline guessing or to aid a social engineering attack. 

\subsubsection{Composition}
\paragraph{Enforce restrictions on characters}
Researchers have shown that having complex password composition rules can make the resulting passwords more difficult to guess \cite{kelley2012guess}. Though simply allowing only long (greater than 16 characters) passwords has a similar effect on guessability and may not cause as much hardship for users  \cite{kelley2012guess}. Having very stringent composition rules does have the effect of limiting the search space an attacker needs to look through. For example, a brute force exhaustive attacker has to search more possibilities for a password with 8 characters made up only of lowercase letters, than for an 8 characters password which has to have two numbers, two uppercase letters, two lower case letters and two symbols. This gap increases further if the user voluntarily chooses from all 95 possible character options.

\subsubsection{Keep your account safe}
\paragraph{Check web pages for SSL}
This task helps users verify that communications to this webpage will be transmitted securely with encryption. This will help to combat phishing and pharming since phishing and pharming sites usually do not use SSL encryption. However, Dhamija et al. found that 23\%  of  their  participants  did  not  look  at  browser-based cues  such  as  the  address  bar,  status  bar  or  security indicators \cite{dhamija2006phishing}.

\paragraph{Manually type URLs}
Manually typing URLs can save a user from a Phishing attack as the user should recognize that the URL is not linking to the correct website. However, manually typing URLs makes a user vulnerable to typo-squatting/URL hijacking \cite{szurdi2014long} e.g., \url{www.goggle.com}. A user is sent to the site with the similar URL which masquerades as the website of the user's intended destination. The site can then ask the user to enter their login details and store them to use on the real site. Thus the user's password is duplicated. 

\paragraph{Keep software updated}
By keeping software updated a user gains protection against vulnerabilities as soon as the patch is released. This can save a user from eavesdropping, side channel and endpoint compromise. %online guessing? 

\paragraph{Log out of public computers}
If a user does not log out of a public computer then the only protection a user has is the moral compass of the next person person who uses that computer. In this way a user's account can already be thought of as in a state of compromise. It is not obvious which of the 11 categories this opportunist attack comes under. We will somewhat arbitrarily place it under Eavesdropping. 

\paragraph{Password protect your phone}
If a phone is password protected then the probability of endpoint compromise is lower.

\subsubsection{Multi-factor authentication}
\paragraph{Use Multi-factor authentication}
As mentioned before multi-factor authentication traditionally involves: \textit{something you are}, \textit{something you know}, and \textit{something you have}. The \textit{something you have} is susceptible to theft. However, if it is stolen the user if still protected by their other authentication factor. Using multi-factor authentication decreases the success of phishing (as second factors are often not subject to replay) and online guessing attacks (as both factors must be guessed). We underline some of the benefits as it depends on which factors the user or organization choose to use. 

\paragraph{Use 2-step verification on phone}
The phone can be stolen or the code can be revealed by eavesdropping or a side channel attack. But again, if the phone is compromised, it is possible that the first step of the authentication process will keep the users' account secure. 2-step verification decreases the success of an online guessing attack and a phishing attack.  

\paragraph{Use for remote accounts}
Without knowledge of a specific second factor it is hard to say what the security effects are. Therefore, depending on what the second factor is, there is the potential for physical theft or endpoint compromise to jeopardize the authentication. The probability of the exchange being eavesdropped is much higher if used for remote accounts.

\subsubsection{Password managers}
\paragraph{Use a password manager}
If we assume the norm is for users to memorize their passwords, then a password manager does not, in its own right, offer additional security. It does greatly reduce the users' memory load and by extension then a user can use as long, random and complex of a password as they wish. Thus this act will increase security but just using the password manager does not guarantee users will increase the complexity of their passwords. A password manager does mean that the user is relying on an external agent to store their passwords and therefore if this agent is compromised then the passwords of all accounts are compromised. Therefore we consider this to be a new way in which the users' password can be duplicated. 

Password managers which automatically fill in the users' credentials with no user interaction do have some corner case vulnerabilities \cite{silver2014password}. Though this same paper shows that a password manager can provide more security that the normal manual typing of the password. But it does depend on the set up of the specific password manager. 

\paragraph{Create long random passwords}
This piece of advice was given in the context of a password manager. ``Configure your password manager to create 30--50 random characters with a mixture of upper- and lower-case letters, numbers, and symbols.'' It has the same benefits as creating a complex long password but without the user memory costs.

\subsubsection{Personal password storage}
\paragraph{Don't store in a computer file.}
An attacker accessing this password file can duplicate the password. %If the laptop or computer is stolen the password file would also be taken.

\paragraph{Write down safely}
Even if the password is stored safely, the very act of writing it down makes it's duplication and physical theft possible. There is discussion as to whether the security risks of writing passwords are in fact very low \cite{schneierwritedown}. And in fact, if users write down passwords, then they may be more confident making stronger password choices \cite{cheswick2013rethinking}\cite{komanduri2011passwords}\cite{herley2009so}.

\paragraph{Don't choose ``remember me''.}
If the ``remember me'' option is not used then if an attacker steals a laptop or computer they should not automatically have access to the accounts on it. It is equivalent to not logging out of an account.

\subsubsection{Reuse}
\paragraph{Never reuse a password}
Reusing passwords has the security disadvantage that if an attacker compromises a password on one site then the password can be used to gain access to other sites. 
This means if passwords are reused then online and offline guessing becomes much easier for an attacker. In fact, if the password is leaked elsewhere the chance of it being compromised for this given organization is just equal to be chance that an attacker tries. 
%phishing and pharming and social engineering attacks?

However, even with different passwords at different sites, the attacker has a good chance of being able to leverage the information from a separate compromised site to mount effective phishing, social engineering and guessing attacks \cite{das2014tangled}. These will be at a higher cost to the attacker though.

\paragraph{Alter and reuse passwords }
Altering and reusing passwords means not directly reusing passwords between sites. It will make a guessing attack necessary for an attacker even if they have access to a password belonging to the same user from a different site. However, Das et al. \cite{das2014tangled} were able to guess approximately 10\% of non-identical password pairs in less than 10 attempts and approximately 30\% in less than 100 attempts. Therefore we mark it as a limited security improvement. 

\paragraph{Don't reuse certain passwords.}
Asking users to not reuse certain passwords is equivalent to saying that a user can reuse some passwords. 

In fact, if we look at the specific advice in this category we can see that most organizations are asking users to not reuse the password for \emph{their} site. This does provide some security advantage as the attacker will not be able to directly access the protected account using the revealed password. But, as with ``don't reuse you passwords'' we know that an attacker can still leverage information from other compromised sites to attempt phishing, social engineering and guessing attacks.

\subsubsection{Sharing}
\paragraph{Never share your password}
In the process of sharing a password it could be eavesdropped. Not allowing users to share their passwords also helps to protect against social engineering. Though this is through the form of user education.
